# Supplementary material for: Thompson Sampling-like Algorithms for Stochastic Rising Bandits
Source: arXiv:2505.12092 source file (2025-05-20)
Supplement: Supplementary file 1 [file appendix.tex]

\onecolumn
\appendix

\section{Proofs and Derivations}\label{apx:proofs}
In this appendix, we provide the complete proofs and derivations we have omitted in the main paper.

\subsection{Further Definitions}
Given the existence of $T^* $ as defined in Assumption \ref{ass:env2}, it will be useful for the purpose of analysis to define (assuming $\max_{i \in \dsb{K}}\{\Delta_i(+\mathcal{1},0)\}$ exists finite):
\begin{equation}\label{eq:costante}
	c =\frac{\max_{i \in \dsb{K}}\{\Delta_i(+\mathcal{1},0)\}}{\min_{i \neq i^*(T') ,T'\in \dsb{T^*-1}} \{\overline{\Delta}_i(\sigma',T'),\overline{\Delta}_i(T^*,+\mathcal{1})\}},
\end{equation}
where $\sigma'\in \dsb{\sigma(T'),T'}$.

\begin{restatable}[Wald's Identity for Rising Bandits]{lemma}{wald}\label{lemma:wald}
	For every algorithm $\mathfrak{A}$ and learning horizon $T \in \Nat$, it holds that:
	\begin{align}
		R(\mathfrak{A},T) \le \sum_{i=2}^K \Delta_i(T,0)\E[N_{i,T}],
	\end{align}
	where $\Delta_i(T,0) \coloneqq \mu_1(T) - \mu_i(0)$.
\end{restatable}
\begin{proof}
	We start with the usual definition of regret and proceed as follows:
	\begin{align}
		R(\mathfrak{A},T) & = T \overline{\mu}_1 - \E \left[ \sum_{t=1}^T  \mu_{I_t}(N_{I_t,t}) \right] \\
		& =  \E \left[ \sum_{t=1}^T \left(  \mu_1(t) - \mu_{I_t}(N_{I_t,t}) \right) \right] \\
		& = \E \left[ \sum_{t=1}^T  \mu_1(t) - \sum_{j=0}^{N_{1,T}} \mu_1(j) - \sum_{i=2}^K \sum_{j=0}^{N_{i,T}} \mu_{i}(j) \right] \\
		& = \E \left[ \sum_{j=N_{1,T}+1}^T  \mu_1(j) - \sum_{i=2}^K \sum_{j=0}^{N_{i,T}} \mu_{i}(j) \right] \\
		& \le \E \left[ \sum_{i=2}^K \sum_{j=0}^{N_{i,T}} \left( \mu_1(T) -  \mu_{i}(j)  \right) \right] \\
		& \le \sum_{i=2}^K \left( \mu_1(T) - \mu_i(0) \right) \E \left[ \sum_{j=0}^{N_{i,T}} 1  \right].
	\end{align}
	
\end{proof}

\begin{restatable}{lemma}{assass}\label{lemma:assass}
	Assumption~\ref{ass:env2} entails the fact that $\overline{\Delta}_i(T,T)$ are lower bounded with:
	\begin{align*}
		c =\frac{\max_{i \in \dsb{K}}\{\Delta_i(+\mathcal{1},0)\}}{\min_{i \neq 1 ,T'\in \dsb{T^*-1}} \{\overline{\Delta}_i(T',T'),\overline{\Delta}_i(T^*,+\mathcal{1})\}}.
	\end{align*}
\end{restatable}
\begin{proof}
	Let us assume now it the arms dynamics are such that it exists a finite time horizon $T^*$ defined as:
	\begin{align}
		\overline{\mu}_1(T^*)>\overline{\mu}_i(+\mathcal{1}), \forall i \neq 1,
	\end{align}
	where we used the fact that for $T > T^*$ the arm identified by the theorem is the optimal arm ($1 = i^*$). Informally, there is a finite time over which the best arm will not change anymore, we can devise a finite grid of values for every $T$ and every $i$ of $\overline{\Delta}_i(T,T)$, up to $T^*$, for $T^*$ we will consider $\overline{\Delta}_i(T^*,\mathcal{1})$. Indeed we notice that $\overline{\Delta}_i(T^*,\mathcal{1})$ is smaller than any possible permutation (as the arms' average is rising) for any horizon $T\ge T^*$, i.e by definition $\forall$ $\epsilon, \text{ } \eta\ge 0$:
	\begin{equation}
		\overline{\Delta}_i(T^*+\eta,T^*+\epsilon) \ge \overline{\Delta}_i(T^*,T^*+\epsilon)\ge \overline{\Delta}_i(T^*,\mathcal{1}),
	\end{equation}
	so any constant that were to bound $\frac{\max_{i \in \dsb{K}}\{\Delta_i(+\mathcal{1},0)\}}{\overline{\Delta}_i(T^*,\mathcal{1})}$ would also bound all the infinite values $\frac{\max_{i \in \dsb{K}}\{\Delta_i(+\mathcal{1},0)\}}{\overline{\Delta}_i(T^*+\eta,T^*+\epsilon)}$. 
	Then $c$ is well defined, and it is possible to define it as (assuming $\max_{i \in \dsb{K}}\{\Delta_i(+\mathcal{1},0)\}$ exists finite):
	\begin{equation} \label{eq:cdefin}
		c =\frac{\max_{i \in \dsb{K}}\{\Delta_i(+\mathcal{1},0)\}}{\min_{\{i \neq 1 ,T'\in \dsb{T^*-1}\} }\{\overline{\Delta}_i(T',T'),\overline{\Delta}_i(T^*,\mathcal{1})\}},
	\end{equation}
\end{proof}

\subsection{Proofs of Section~\ref{sec:AnalysisBetaTS}}

\mf*
\begin{proof}
    Let $N_{1,t} = j$, $S_{1,t}= s$. Then,
As shown by~Agrawal et al.~\cite{agrawal2012analysis}, $p_{i,t}$ can be written as:
    $$p_{i,t} = \Prob(\theta_{1,t} > y_i) = F^B_{j+1,y_i}(s).$$
    For ease of notation, let us denote $X' \sim \text{PB}(\underline{\mu}_{1}(j))$ and $X\sim \text{Bin}(j, x)$.
We are now interested in finding if it does exist a number of trials $j$ such that:
%\begin{align}\label{eq:condition}
%    (**)=\mathbb{E}_{\underline{\mu}_{1}(j)}^{\text{PB}}\left[\frac{1}{F_{j+1, y_i}^B}\right]\leq\mathbb{E}_{\overline{\mu}_{1}(\sigma)}^{\text{Bin}}\left[\frac{1}{F_{j+1, y_i}^B}\right]=(*).
%\end{align}
\begin{align}\label{eq:condition111}
	(**)=\mathbb{E}\left[\frac{1}{F_{j+1, y_i}^B(X')}\right]\leq\mathbb{E}\left[\frac{1}{F_{j+1, y_i}^B(X)}\right]=(*).
\end{align}
    We notice that the PMF of a binomial distribution is discrete log-concave (see Lemma~\ref{lemma:con}), so that let $Y$ be a binomial random variable, we will have:
\begin{equation}\label{eq;conbin}
	p_Y(i+1)^2 \geq p_Y(i) p_Y(i+2),
\end{equation}
so by Lemma~\ref{lemma:logcon} used with $\alpha = 1$ and $r = \infty$, and $q$ being the probability mass function of the binomial distribution (more in-depth $q(x) = p(-x)$ in Lemma~\ref{lemma:logcon}) we find that the CDF of the binomial is discrete log-concave on $\mathbb{Z}$ too (indeed the theorems cited above state that if the probability mass function of an integer-valued random variable is discrete log-concave as a function on $\mathbb{Z}$, then the corresponding CDF ($F^B$ in our notation) is also discrete log-concave as a function on $\mathbb{Z}$) and so by definition, omitting superscripts and subscripts,  $1 / F$ is discrete log-convex (same inequality of \ref{eq;conbin} with different sign) on the set $S:=\{0,\ldots j+1\}$ of all atoms of the distribution. So, $1 / F$ is strictly discrete convex on $S$. Indeed by proving the discrete log-convexity of $\frac{1}{F}$ we have proved that:
\begin{equation}
	\left(\frac{1}{F(x+1)}\right)^2\leq\frac{1}{F(x+2)}\frac{1}{F(x)},
\end{equation}
by applying the logarithm, we obtain the following:
\begin{equation}
	2\log\left(\frac{1}{F(x+1)}\right)\leq \log\left(\frac{1}{F(x+2)}\frac{1}{F(x)}\right),
\end{equation}
then, since the logarithm is monotonic, increasing:
\begin{equation}
	\left(\frac{1}{F(x+1)}\right)\leq \left(\frac{1}{F(x+2)}\right)^{\frac{1}{2}}\left(\frac{1}{F(x)}\right)^{\frac{1}{2}}.
\end{equation}
Using the AM-GM inequality, we obtain:
\begin{align}
	\left(\frac{1}{F(x+1)}\right)<  \frac{1}{2}\left(\frac{1}{F(x+2)}\right)+ \frac{1}{2}\left(\frac{1}{F(x)}\right) \\ 
	2\left(\frac{1}{F(x+1)}\right)<\left(\frac{1}{F(x+2)}\right)+\left(\frac{1}{F(x)}\right),
\end{align}
where the inequality is strict since $\frac{1}{F(x+2)} < \frac{1}{F(x)}$ for $x\in\{0, \ldots, j-1\}$, and, therefore, $\frac{1}{F(x+2)} \neq \frac{1}{F(x)}$. We use Lemma~\ref{lemma:hoeffpomp} over the above quantities, which implies that $\forall$ $j$ we will have that the expected value of the term of our interest for a Poisson-Binomial process with a certain average of the probabilities of the success at each trial is always smaller than the one of a Binomial process with probability of success at each trial equal to the average of the probabilities of success at each trial of the real Poisson-binomial process (when considered for the same number of trials). To show that $(*) \leq (**)$ for any $j$ such that $\overline{\mu}_1(j)\ge x$ we need to prove that the expected value of $\frac{1}{F}$ considered for a Binomial process with mean $\overline{\mu}_{1}(j)$ is smaller than the expected value of $\frac{1}{F}$ for a Binomial Process with mean $x$. 

We apply Lemma~\ref{lemma:change} stating that for a non-negative random variable (like ours $1/{F_{j+1, y_i}^B}$), the expected value can be computed as:
\begin{align}
	\mathbb{E}\left[\frac{1}{F_{j+1, y_i}^B}\right]=\int_{0}^{+\infty}\Prob\left(\frac{1}{F_{j+1, y_i}^B}\ge y\right) \de y.
\end{align}
Let $X''\sim \text{Bin}(j, \overline{\mu}_1(j))$. Thus, we have:
\begin{align}
	\Prob\left(\frac{1}{F_{j+1, y_i}^B} \ge y \right)& = \Prob(X''=0)+\Prob(X''=1)+\ldots+\Prob\left(X''=\left(\frac{1}{F_{j+1,y_i}^B}\right)^{-1}(y) \right)\\
	& =\Prob\left(X''\leq \underbrace{\left(\frac{1}{F_{j+1,y_i}^B}\right)^{-1}(y) }_{\text{$\eqqcolon k_j(y)$}} \right),
\end{align}
and
\begin{align}
	\Prob\left(\frac{1}{F_{j+1, y_i}^B} \ge y \right)& = \Prob(X=0)+\Prob(X=1)+\ldots+\Prob\left(X=\left(\frac{1}{F_{j+1,y_i}^B}\right)^{-1}(y) \right)\\
	& =\Prob\left(X\leq \underbrace{\left(\frac{1}{F_{j+1,y_i}^B}\right)^{-1}(y) }_{\text{$\eqqcolon k_j(y)$}} \right),
\end{align}
where the inverse is formally defined as follows:
\begin{align}
	\left(\frac{1}{F_{j+1,y_i}^B}\right)^{-1}(y) \coloneqq \max\left\{ s : y \le \frac{1}{F_{j+1,y_i}^B(s)} \right\}.
\end{align}
Thus, the above condition in Equation~\eqref{eq:condition111} becomes:
\begin{align}\label{eq:condtion2}
	\int_{0}^{+\infty}\Prob(X''\leq k_j(y))\de y&\leq \int_{0}^{+\infty}\Prob(X\leq k_j(y))\de y.
\end{align}
A sufficient condition to ensure that the condition in Equation~\eqref{eq:condtion2} is that:
\begin{equation} \label{eq:condition3}
	\Prob(X'\le m)\le \Prob(X\le m), \forall m \iff\Prob(X'\ge m)\ge \Prob(X\ge m), \forall m.
\end{equation}

Let us recall the concept of stochastic order~\citep{boland2002stochastic,boland2004sstochasticordertesting,marshall2011inequalities}) that is often useful in comparing random variables. For two random variables $U$ and $V$, we say that $U$ is greater than $V$ in the usual stochastic order, and we denote it with $U\ge_{\text{st}}V$, when $\Prob(U\ge m) \ge \Prob(V \ge m), \forall m$.
Thus, if we have that $X' \ge_{\text{st}} X$ we would have that also Equation~\eqref{eq:condition3} holds too. It has been shown by ~\cite{boland2002stochastic} (Lemma \ref{lemma:stochastic}) that the condition for that to happen when $X'$ and $X$ are binomial distribution  with mean $\mu'$ and $\mu$ is that $\mu'\ge \mu$.
%{\color{red} MARCO: forse ci sta bene definirlo senza mettere che j appartenga tra 0 e T, perchè esiste comuqunque se la dinamica continua, al di la del fatto che non ci arriviamo, questo lo si può usare per dire che se c'è un orizzonte temporale entro il quale il braccio migliore non cambia più possiamo estendere per tutti gli orizzonti finiti (anche minori di xi la somma fino a xi e dire che è una costante e dunque evolviamo lnT+const}:
By doing that we showed that for any $j$ such that $\overline{\mu}_1(j)\ge x$:
\begin{equation}
	\mathbb{E}_{\text{PB($\underline{\mu}_1(j)$)}}\left[\frac{1}{F_{j+1,y}}\right]\leq \mathbb{E}_{\text{Bin(j,$\overline{\mu}_1(j)$)}}\left[\frac{1}{F_{j+1,y}}\right]\leq \mathbb{E}_{\text{Bin($j,x$)}}\left[\frac{1}{F_{j+1,y}}\right],
\end{equation}  
concludes the proof.
\end{proof}

\ts*

\begin{proof}
For every suboptimal arm $i \in \dsb{2,K}$, let us define the thresholds $x_i$ and $ y_i$ s.t.~$\overline{\mu}_{i}(T)< x_i < y_i < \overline{\mu}_{1}(\sigma_i)$. Thanks to the above thresholds, we can define the following events for every $t \in \dsb{T}$:
\begin{itemize}
	\item $E^{\mu}_{i}(t)$ as the event for which $\hat{\mu}_{i,t} \leq x_{i}$;
	\item $E^{\theta}_{i,t}$ as the event for which $\theta_{i,t} \leq y_{i}$, where $\theta_{i,t}$ denotes a sample generated for arm $i$ from the posterior distribution at time $t$, i.e., $\text{Beta}(S_{i,t} + 1, F_{i,t} + 1)$, being $S_{i,t}$ and $F_{i,t}$ the number of successes and failures up to round $t$ for arm $i$ (note that $N_{i,t} = S_{i,t} + F_{i,t}$ and $\mu_{i,t} = S_{i,t}/N_{i,t}$).
\end{itemize}
Moreover, let us denote with $E^{\mu}_{i}(t)^\complement$ and $E^{\theta}_{i}(t)^\complement$ the complementary event $E^{\mu}_{i}(t)$ and $E^{\theta}_{i}(t)$, respectively. Using Lemma~\ref{lemma:wald}, we can rewrite the regret as:
\begin{equation}
	R(\text{\texttt{Beta-TS}},T) \leq \sum_{i=2}^{K} {\Delta_{i}(T,0)} \E[N_{i,T}] =  \sum_{i=2}^{K} {\Delta_{i}(T,0)}\sum_{t=1}^{T}{\Prob(I_t=i)}.
\end{equation}
Let us focus on decomposing the probability term in the regret as follows:
\begin{align}
	\sum_{t=1}^{T}\Prob(I_t=i)  & =\underbrace{ \sum_{t=1}^{T} \Prob(I_t=i,E^{\mu}_{i}(t)^\complement)}_{=: P_A} + \underbrace{\sum_{t=1}^{T} \Prob(I_t=i,E^{\mu}_{i}(t),E^{\theta}_{i}(t)^\complement)}_{=: P_B} \\
	&  \quad + \underbrace{\sum_{t=1}^{T} \Prob(I_t = i, E^{\mu}_{i}(t), E^{\theta}_{i}(t))}_{=: P_C}.
\end{align}
The three terms correspond to the case of:
\begin{itemize}
	\item (i) having a poor estimation of the mean for arm $i$ (i.e., $P_A$);
	\item (ii) having a good estimation of the mean and having sampled a large value for the arm $i$ posterior sample (i.e., $P_B$);
	\item (iii) having a good estimate for the mean of the reward and having sampled a small value for the posterior sample of arm $i$ (i.e., $P_C$).
\end{itemize}
Let us analyze each term separately.

\paragraph{Term A}
Let $\tau_k \in \dsb{T}$ denote the round at which we pull the arm $i$ for the $k$-th time (we are omitting the dependence on the arm index $i$ to avoid heaving the notation).
In what follows, we let the sum run to times that can be greater than $T$.
We have:
\begin{align}
	P_A &= \sum_{t=1}^{T} \Prob(I_t =i, E^{\mu}_{i}(t)^\complement) \\
	& \leq \mathbb{E} \left[ \sum_{k=1}^{T} \sum_{t=\tau_k+1}^{\tau_{k+1}} \mathds{1} \left\{ I_t=i \right\} \mathds{1} \left\{ E^{\mu}_{i}(t)^\complement \right\} \right]\\
	& \leq \mathbb{E} \left[ \sum_{k=0}^{T-1} \mathds{1} \left\{ E^{\mu}_{i}(\tau_k+1)^\complement\right\} \underbrace{\sum_{t=\tau_k+1}^{\tau_{k+1}} \mathds{1} \left\{ I_t=i \right\}}_{= 1} \right]  \label{l:this001} \\
	&  =\mathbb{E} \left[ \sum_{k=0}^{T-1} \mathds{1} \left\{ E^{\mu}_{i}(\tau_k+1)^\complement) \right\} \right]\\
	&\leq 1 + \mathbb{E} \left[ \sum_{k=1}^{T-1} \mathds{1} \left\{ E^{\mu}_{i}(\tau_k+1)^\complement \right\} \right] = 1 + \sum_{k=1}^{T-1} \underbrace{\Prob ( E^{\mu}_{i}(\tau_k+1)^\complement)}_{=:P_D},
\end{align}
where Equation~\eqref{l:this001} follows from observing that the indicator function is $1$ in a single round in the inner summation.
Let us notice that thanks to the definition of the event $E^{\mu}_{i}(\tau_{k}+1)$, the term $P_D$ corresponds to the probability that $\hat{\mu}_{i,\tau_k} > x_i$ after exactly $k$ pulls (which is not a random variable).
Thus, using Lemma~\ref{lemma:chernoff} with $\lambda = x_i - \overline{\mu}_{i}(k)$ and recalling that $\E[\hat{\mu}_{i,\tau_k} ]=\overline{\mu}_{i}(k)$, we have:
\begin{align}
	P_D & = \Prob ( \hat{\mu}_{i,\tau_k}  > x_i) = \Prob(\hat{\mu}_{i,\tau_k}  > \overline{\mu}_{i}(k) - \overline{\mu}_{i}(k) + x_i)\\
	& \leq \exp \left( -k \ d(x_i, \overline{\mu}_{i}(k)) \right) \leq \exp \left( -k \ d(x_i, \overline{\mu}_{i}(T)) \right),
\end{align}
where $d(a, b) = a \ln{\frac{a}{b}} + (1 - a) \ln{\frac{1-a}{1-b}}$ is the Kullback-Leiber distance between two Bernoulli variables with expected value $a$ and $b$, and the last inequality follows from the fact that $x_i > \mu_i(T)$.
This implies that:
\begin{equation}
	P_A \leq 1 + \sum_{k=1}^{T-1} \exp \left( -k \ d(x_i, \overline{\mu}_{i}(T)) \right) \leq 1 + \frac{1}{d(x_i, \overline{\mu}_{i}(T))},
\end{equation}
where the last inequality follows from bounding the summation with the corresponding integral.

\paragraph{Term B}
Let us focus on the summands of the term $P_B$ of the regret. To this end, let $(\mathbb{F}_{t-1})_{t \in \dsb{T}}$ be the canonical filtration. We have:
\begin{align}
	\Prob( I_t = i, E^{\theta}_{i}(t)^\complement|E^{\mu}_{i}(t),\mathbb{F}_{t-1})  & \leq \Prob(\theta_{i,t}>y_{i}|\hat{\mu}_{i,t} \leq x_{i}, \mathbb{F}_{t-1}) \\
	& = \Prob \left( \text{Beta} \left( \hat{\mu}_{i,t} N_{i,t} + 1, (1 - \hat{\mu}_{i,t}) N_{i,t} + 1 \right) > y_{i} | \hat{\mu}_{i,t} \leq x_{i} \right) \label{line:line}\\
	& \leq \Prob \left( \text{Beta} \left( x_{i} N_{i,t} + 1, (1 - x_{i}) N_{i,t} + 1 \right) > y_{i} \right) \\
	& \leq F^{B}_{N_{i,t},y_{i}}\big(x_{i}N_{i,t}\big) \leq \exp \left( - N_{i,t} d(x_{i}, y_{i}) \right),
\end{align}
where the last inequality follows from the generalized Chernoff-Hoeffding bounds  (Lemma~\ref{lemma:chernoff}) and the Beta-Binomial identity (Fact 3 of~\cite{agrawal2017near}). Equation~\eqref{line:line} was derived by exploiting the fact that on the event $E^{\mu}_{i}(t)$ a sample from $\text{Beta} \left( x_{i} N_{i,t} + 1, (1 - x_{i}) N_{i,t} + 1 \right) $ is likely to be as large as a sample from $Beta( \hat{\mu}_{i,t} N_{i,t}(t) + 1, (1 - \hat{\mu}_{i,t})N_{i,t} + 1 )$, reported formally in Fact~\ref{lem:betabin}.
Therefore, for $t$ such that $N_{i,t} > L_i(T )$, where $L_i(t) \coloneqq \frac{\log{T}}{d(x_i,y_i)}$ we have:
\begin{equation}
	\Prob(I_t=i,E^{\theta}_{i}(t)^\complement|E^{\mu}_{i}(t),\mathbb{F}_{t-1})\leq\frac{1}{T}.
\end{equation}

Let $\tau$ be the largest round until $N_{i,t} \leq L_i(T )$, then:
\begin{align}
	P_B & = \sum_{t=1}^{T}\Prob\big(I_t=i,E^{\mu}_{i}(t),E^{\theta}_{i}(t)^\complement \big)\leq \sum_{t=1}^{T}\Prob\big(I_t=i,E^{\theta}_{i}(t)^\complement |E^{\mu}_{i}(t)\big)\\
	& =\mathbb{E}\Big[\sum_{t=1}^{T}\Prob(I_t=i,E^{\theta}_{i}(t)^\complement|E^{\mu}_{i}(t),\mathbb{F}_{t-1}) \Big]\\
	& = \mathbb{E}\Big[ \sum_{t=1}^{\tau} \Prob(I_t=i,E^{\theta}_{i}(t)^\complement|E^{\mu}_{i}(t),\mathbb{F}_{t-1})+\sum_{t=\tau+1}^{T} \Prob(I_t=i,E^{\theta}_{i}(t)^\complement|E^{\mu}_{i}(t),\mathbb{F}_{t-1})\Big]\\
	& \leq \mathbb{E}\Big[ \sum_{t=1}^{\tau} Pr(I_t=i,E^{\theta}_{i}(t)^\complement|E^{\mu}_{i}(t),\mathbb{F}_{t-1})\Big]+\E \left[ \sum_{t=\tau+1}^{T} \frac{1}{T} \right] \\
	& \leq \mathbb{E}\Big[ \sum_{t=1}^{\tau} \Prob(I_t=i,E^{\theta}_{i}(t)^\complement|E^{\mu}_{i}(t),\mathbb{F}_{t-1})\Big]+1\\
	& = \mathbb{E}\Big[ \sum_{t=1}^{\tau} \mathds{1} (I_t=i)\Big]+1\\
	& \leq L_i(T) + 1.
\end{align}

\paragraph{Term C}
For this term, we shall use Lemma~1 by~\cite{agrawal2017near}. Let us define $p_{i,t} = \Prob(\theta_{1,t} > y_i | \mathbb{F}_{t-1})$. We have:
\begin{equation}
	\Prob(I_t = i, E^{\mu}_{i}(t), E^{\theta}_{i}(t) | \mathbb{F}_{t-1}) \leq \frac{1-p_{i,t}}{p_{i,t}} \Prob(I_t = 1, E^{\mu}_{i}(t), E^{\theta}_{i}(t)|\mathbb{F}_{t-1}).
\end{equation}
Thus, we can rewrite the term $P_C$ as follows:
\begin{align}
	P_C  & = \sum_{t=1}^{T}\Prob(I_t=i,E^{\mu}_{i}(t),E^{\theta}_{i}(t)) \\
	& = \sum_{t=1}^{T} \mathbb{E}[\Prob(I_t=i,E^{\mu}_{i}(t),E^{\theta}_{i}(t)|\mathbb{F}_{t-1})] \\
	&\leq \sum_{t=1}^{T}\mathbb{E}\bigg[\mathbb{E}\bigg[\frac{1-p_{i,t}}{p_{i,t}}\mathds{1}(I_t=1,E^{\mu}_{i}(t),E^{\theta}_{i}(t))\bigg|\mathbb{F}_{t-1}\bigg]\bigg] \\
	&\leq\sum_{t=1}^{T}\mathbb{E}\bigg[\frac{1-p_{i,t}}{p_{i,t}}\mathds{1}(I_t=1,E^{\mu}_{i}(t),E^{\theta}_{i}(t))\bigg].\\
\end{align}
Let $\tau_k$ denote the time step at which arm $1$ is played for the $k$-th time (notice we allow the sum to run trough times bigger than the learning horizon $T$), and let $\tau_0 = 0$:
\begin{align}
	P_C &\leq \sum_{k=0}^{T-1}\mathbb{E}\bigg[\frac{1-p_{i,\tau_{k}+1}}{p_{i,\tau_{k}+1}}\sum_{t=\tau_k+1}^{\tau_{k+1}}\mathds{1}(I_t=1,E^{\mu}_{i}(t),E^{\theta}_{i}(t))\bigg]\\
	&\leq\sum_{k=0}^{T-1}\mathbb{E}\bigg[\frac{1-p_{i,\tau_k+1}}{p_{i,\tau_k+1}}\bigg], \label{eq:fixed}
\end{align}
where the inequality in Equation~\eqref{eq:fixed} uses the fact that $p_{i,t}$ is fixed, given $\mathbb{F}_{t-1}$. Then, we observe that $p_{i,t} = \Prob(\theta_{1,t} > y_i |\mathbb{F}_{t-1})$
changes only when the distribution of $\theta_{1,t}$ changes, that is, only on the time step after each play of the first arm. Thus, $p_{i,t}$ is the same at all time steps $t \in \{\tau_k+1, \dots , \tau_{k+1}\}$, for every $k$. Finally, bounding the probability of selecting the optimal arm by $1$ we have:
\begin{equation}
	P_C \leq \sum_{k=0}^{T-1}\mathbb{E} \left[ \frac{1}{p_{i,\tau_k+1}} - 1 \right].
\end{equation}

Let $N_{1,t} = j$, $S_{1,t}= s$. Then,
$$p_{i,t} = \Prob(\theta_{1,t} > y_i) = F^B_{j+1,y_i}(s)$$
due to the relation that links the Beta and the Binomial distributions (Fact 3 of~\cite{agrawal2017near}). Let $\tau_j + 1$ denote the time step after the $j$-th play of the optimal arm. Then, $N_{1,\tau_j + 1} = j$. We do notice a sensible difference with respect to the stationary case. Indeed, the number of successes after $j$ trial is not distributed anymore as a binomial distribution. Instead, it can be described by a Poisson-Binomial distribution $\text{PB}(\underline{\mu}_{1}(j))$ where the vector $\underline{\mu}_{1}(j)=(\mu_{1}(1),\ldots,\mu_{1}(j))$, and $\mu_{1}(m)$ represents the probability of success of the best arm at the $m$-th trial. The probability of having $s$ successful trials out of a total of $j$ trials can be written as follows~\citep{wang1993poissobinomial,poisson2019english}:
\begin{align}
	f_{j,\underline{\mu}_{1}(j)}(s)=\sum_{A \in F_s} \prod_{m \in A}\mu_{1}(m)\prod_{m' \in A^c}(1-\mu_{1}(m')),   
\end{align}
where $F_{s}$ is the set of all subsets of $s$ integers that can be selected from $\dsb{j}$. $F_s$ by definition will contain $\frac{j!}{(j-s)!s!}$ elements, the sum over which is infeasible to compute in practice unless the number of trials $j$ is small. A useful property of $f$ is that it is invariant to the order of the elements in $\underline{\mu}_{1}(j)$. Moreover, we define density function of the binomial of $j$ trials and mean $\overline{\mu}_{1}(j)$, i.e., $\text{Bin}(j,\overline{\mu}_{1}(j))$, as:
\begin{align}
	f_{j,\overline{\mu}_{1}(j)}(s) = \binom{j}{s} \overline{\mu}_{1}(j)^s (1-\overline{\mu}_{1}(j))^{j-s}.
\end{align}
By applying the change of measure argument of Lemma~\ref{lemma:changeMeasure}, we have:
\begin{align}
	\mathbb{E}\left[\frac{1}{F_{j+1, y_i}^B} \right] &= \underbrace{\sum_{s=0}^{j} \frac{f_{j,\underline{\mu}_{1}(j)}(s)}{F_{j+1, y_i}^B(s)}}_{\textbf{$(**)$}}\leq \left(\frac{1}{(1-y_i)^{j+1}}-1\right)\delta_{\text{TV}}\left(\text{PB}(\underline{\mu}_{1}(j)),\text{Bin}(j,\overline{\mu}_{1}(\sigma_i))\right)+ \underbrace{\sum_{s=0}^{j} \frac{f_{j,\overline{\mu}_{1}(\sigma)}(s)}{F_{j+1, y_i}^B(s)}}_{\textbf{$(*)$}},
\end{align}
where $\delta_{TV}(P,Q) \coloneqq \sup_{A\in\mathcal{F}}{\big|P(A)-Q(A)\big|}$ is the total variation between the probability measures $P$ and $Q$ (assuming they are defined over a measurable space $(\Omega,\mathcal{F})$, having observed that, using the notation of Lemma~\ref{lemma:changeMeasure}:
\begin{align}
	& b= \max_{s \in \dsb{0,j}} \frac{1}{F^B_{j+1,y_i}(s)} = \frac{1}{F^B_{j+1,y_i}(0)} =\frac{1}{\Prob(\text{Bin}(j+1,y_i)=0)} =  \frac{1}{(1-y_i)^{j+1}}, \\
	& a =\min_{s \in \dsb{0,j}} \frac{1}{F^B_{j+1,y_i}(s)} = \frac{1}{F^B_{j+1,y_i}(j)} =\frac{1}{\Prob(\text{Bin}(j+1,y_i)\le j)} \ge \frac{1}{\Prob(\text{Bin}(j+1,y_i)\le j+1)} = 1.  
\end{align}
For ease of notation, let us denote $X' \sim \text{PB}(\underline{\mu}_{1}(j))$ and $X\sim \text{Bin}(j, \overline{\mu}(\sigma_i))$.
%we denote the expected values with respect to the Poisson-Binomial distribution and the Binomial distribution respectively as $\mathbb{E}_{\underline{\mu}_{1}(j)}^{\text{PB}}[\cdot]$ and $\mathbb{E}_{\overline{\mu}_{1}(j)}^{\text{Bin}}[\cdot]$, respectively.
We are now interested in finding if it does exist a minimum number of trials $j \in \dsb{0,T}$ such that:
%\begin{align}\label{eq:condition}
%    (**)=\mathbb{E}_{\underline{\mu}_{1}(j)}^{\text{PB}}\left[\frac{1}{F_{j+1, y_i}^B}\right]\leq\mathbb{E}_{\overline{\mu}_{1}(\sigma)}^{\text{Bin}}\left[\frac{1}{F_{j+1, y_i}^B}\right]=(*).
%\end{align}
\begin{align}\label{eq:condition1}
	(**)=\mathbb{E}\left[\frac{1}{F_{j+1, y_i}^B(X')}\right]\leq\mathbb{E}\left[\frac{1}{F_{j+1, y_i}^B(X)}\right]=(*).
\end{align}

Thus, using Lemma~\ref{lemma:techlemma}, we conclude that:
\begin{equation}
	\mathbb{E}\left[\frac{1}{F_{j+1,y}}\right]\leq
	\begin{cases}
		\Big(\frac{1}{(1-y_i)^{j+1}}-1\Big)\delta_{\text{TV}}(\text{PB}(\underline{\mu}_{1}(j)),\text{Bin}(j,\overline{\mu}_{1}(\sigma_i)))+ \sum_{s=0}^{j} \frac{f_{j,\overline{\mu}_{1}(\sigma_i)}(s)}{F_{j+1, y_i^B}(s)} & \text{if } 0 \le j<\sigma_i \\
		%\Big(\frac{1}{(1-y_i)^{j+1}}-1\Big)\delta_{\text{TV}}(\text{PB}(\underline{\mu}_{1}(j)),\text{Bin}(j,\overline{\mu}_{1}(j)))+ \sum_{s=0}^{j} \frac{f_{j,\overline{\mu}_{1}(\sigma_i)}(s)}{F_{j+1, y_i^B}(s)} & \text{if } \sigma_i \le j<\xi_i \\
		\sum_{s=0}^{j} \frac{f_{j,\overline{\mu}_{1}(\sigma_i)}(s)}{F_{j+1, y_i}(s)} & \text{if } j\ge\sigma_i \\
	\end{cases}
\end{equation}
Where the total variation terms can be bounded by Lemma \ref{lemma:delta} (imposing $s=0$) and Lemma \ref{lemma:deltadistance} in the auxiliary lemmas. From Lemma 2.9 by~\cite{agrawal2017near}, we have that:
\begin{align}
	\sum_{s=0}^{j} \frac{f_{j,\overline{\mu}_{1}(\sigma_i)}(s)}{F_{j+1, y_i}(s)}-1 \leq
	\begin{cases}
		\frac{3}{\Delta_i'} & \text{if } j<\frac{8}{\Delta_i'}\\
		\Theta\left(e^{-\frac{\Delta_i^{'2}j}{2}}+\frac{e^{-D_i j}}{(j+1)\Delta_i'^{2}}+\frac{1}{e^{\Delta_i'^{2}\frac{j}{4}}-1}\right) & \text{if } j\ge\frac{8}{\Delta_i'}
	\end{cases},
\end{align}
where $\Delta_i'=\overline{\mu}_{1}(\sigma_i)-y_i$ and $D_i=y_i\log{\frac{y_i}{\overline{\mu}_{1}(\sigma_i)}}+(1-y_i)\log{\frac{1-y_i}{1-\overline{\mu}_{1}(\sigma_i)}}$. Thus, summing over all $j$s and using the big-Oh notation to hide all functions of the $\mu_i$s and $\Delta_i'$s, we obtain:
\begin{align}
	\sum_{j=0}^{T-1}\left(\sum_{s=0}^{j}\frac{f_{j,\overline{\mu}_{1}(\sigma_i)}(s)}{F_{j+1, y_i}(s)}-1\right)& \leq \frac{24}{\Delta_i'^2}+\sum_{j\ge\frac{8}{\Delta_i'}}\Theta \left(e^{-\frac{\Delta_i^{'2}j}{2}}+\frac{e^{-D_i j}}{(j+1)\Delta_i'^{2}}+\frac{1}{e^{\Delta_i'^{2}\frac{j}{4}}-1}\right) \\
	& \le  \frac{24}{\Delta_i'^{2}}+\Theta\left(\frac{2}{\Delta_i'^{2}}+\frac{1}{\Delta_i'^{2}D_i}+\frac{1}{\Delta_i'^{4}}\right) = O(1).
\end{align}
which, summing all the contributions to the regret, provides the final result.
\end{proof}
\tscor*
\begin{proof}
   If the arms dynamics is such that exists a finite time horizon $T^*$ defined as:
	\begin{align}
		\overline{\mu}_1(T^*)>\overline{\mu}_i(+\mathcal{1}),\text{ } \forall i \neq 1,
	\end{align}
	i.e., there exists a finite time over which the best arm will not change anymore, we can devise a finite grid of values for every $T$ and every $i$ of $\overline{\Delta}_i(\sigma(T), T)$ (we have taken $\sigma(T)$ for the sake of argument, notice that for every $T$ we could choose any $\sigma \in \dsb{\sigma(T),T}$) up to $T^*$, for $T^*$ we will consider $\overline{\Delta}_i(T^*,\mathcal{1})$. Then, it is possible to define a constant $c$ as in \ref{eq:costante}. Indeed, notice that for all $T \ge T^*$, taking in what we have proved earlier $\sigma=T^*$ for every time horizon $T\ge T^*$, the sum of the total variation distances becomes a constant with respect to the time horizon $T$ and substituting in the result for the online regret we obtain for $T\ge T^*$, $\Delta_i{(T^*,T)}$ with $\Delta_i{(T^*,\mathcal{1})}$:
	\begin{align}
		R(\text{\texttt{Beta-TS}},T) \le O \Bigg( \sum_{i=2}^K \Delta_i(T,0) \Big( (1+\epsilon) \frac{\log (T)}{d(\overline{\mu}_i(\mathcal{1}), \overline{\mu}_1(T^*))} 
		+&\overbrace{\frac{1}{d(x_i,\overline{\mu}_i(\mathcal{1}))}}^{(*)}+ \nonumber \\
		+&  \underbrace{\sum_{j=1}^{T^*-1}\frac{\delta_{\text{TV}}(\text{PB}(\underline{\mu}_{1}(j)),\text{Bin}(j,\overline{\mu}_{1}(T^*)) }{(1-\overline{\mu}_1(T^*))^{j+1}} 
			\Big)}_{(**)}  \Bigg),       
	\end{align}
	Notice that for all $T \ge T^{*}$ we have that both $(*)$ and $(**)$ are constant with $T$. So, neglecting these terms, we obtain:
	\begin{equation}
		R(\text{\texttt{Beta-TS}},T) \le O \Bigg( \sum_{i=2}^K \Delta_i(T,0) \Big( (1+\epsilon) \frac{\log (T)}{d(\overline{\mu}_i(\mathcal{1}), \overline{\mu}_1(T^*))}\Big)\Bigg)   
	\end{equation}
	Using Pinsker's inequality and by definition of $c$, we obtain:
	\begin{equation}\label{eq:ridts}
		R(\text{\texttt{Beta-TS}},T) \le O \Bigg( \sum_{i=2}^K c\overline{\Delta}_i(T^*,\mathcal{1}) \Big( (1+\epsilon) \frac{\log (T)}{2(\overline{\mu}_i(\mathcal{1})- \overline{\mu}_1(T^*))^2}\Big)\Bigg)    
	\end{equation}
	from which we can retrieve the classical instance-independent bound for Thompson Sampling.
	Let's now consider $T\leq T^*$. Rewriting all then we obtain (neglecting the constants):
	\begin{align}
		R(\text{\texttt{Beta-TS}},T) \le O \Bigg( \sum_{i=2}^K \Delta_i(T,0) \Big( \frac{\log (T)}{d(x_i, y_i)} 
		+\overbrace{\frac{1}{d(x_i,\overline{\mu}_i(T))}}^{(*)}+\nonumber\\
		+  \sum_{j=1}^{\sigma(T)-1}\frac{\delta_{\text{TV}}(\text{PB}(\underline{\mu}_{1}(j)),\text{Bin}(j,\overline{\mu}_{1}(\sigma(T))) }{(1-\overline{\mu}_1(\sigma(T)))^{j+1}} 
		\Big) \Bigg),          
	\end{align}
	$(*)$ can be bounded by a constant as we have proven a lower bound for the distances. So we can write thanks to the definition of $c$ in \ref{eq:costante}, and using again Pinsker's inequality:
	\begin{equation}
		R(\text{\texttt{Beta-TS}},T) \le O \Bigg( \sum_{i=2}^K c\overline{\Delta}_i(\sigma(T),T) \Big( \frac{\log (T)}{\overline{\Delta}_i(\sigma(T),T)^2} 
		+  \sum_{j=1}^{\sigma(T)-1}\frac{\delta_{\text{TV}}(\text{PB}(\underline{\mu}_{1}(j)),\text{Bin}(j,\overline{\mu}_{1}(\sigma(T))) }{(1-\overline{\mu}_1(\sigma(T)))^{j+1}} 
		\Big) \Bigg),        
	\end{equation}

	By loosely bounding the total variation by $1$ and noting that the sum over $\sigma(T)$ is a geometric series, we can write neglecting the constants:
	\begin{equation}
		R(\text{\texttt{Beta-TS}},T) \le O \Bigg( \sum_{i=2}^K \overline{\Delta}_i(\sigma(T),T) \Big( \frac{\log (T)}{\overline{\Delta}_i(\sigma(T),T)^2} +\left(\frac{1}{1-\overline{\mu}_1(\sigma(T))}\right)^{\sigma(T)} \Big) \Bigg), 
	\end{equation}
	Similarly to what has been done in~\cite{agrawal2012analysis}, by analyzing the two cases:
	\begin{align}
		\overline{\Delta}_i(\sigma(T),T)&\ge\sqrt{K\frac{\log(T)}{T}},\\
		\overline{\Delta}_i(\sigma(T),T)&\leq\sqrt{K\frac{\log(T)}{T}},
	\end{align}
    we retrieve the final result.
\end{proof}

\clearpage
\subsection{Proofs of Section~\ref{sec:AnalysisGTS}}

\gts*
{
\begin{proof}
For every suboptimal arm $i \in \dsb{2,K}$, let us define the thresholds $x_i$ and $ y_i$ s.t.~$\overline{\mu}_{i}(T)< x_i < y_i < \overline{\mu}_{1}(\sigma_i)$. Thanks to the above thresholds, we can define the following events for every $t \in \dsb{T}$:
\begin{itemize}
    \item $E^{\mu}_{i}(t)$ as the event for which $\overline{\hat{\mu}}_{i,t} \leq x_{i}$;
    \item $E^{\theta}_{i,t}$ as the event for which $\theta_{i,t} \leq y_{i}$, where $\theta_{i,t}$ denotes a sample generated for arm $i$ from the posterior distribution at time $t$, i.e., $\mathcal{N}(\overline{\hat{\mu}}_{i,t},\frac{1}{\gamma N_{i_t,t}})$, being $N_{i_t,t}$  of trials at time $t$ for arm $i_t$.
\end{itemize}
Moreover, let us denote with $E^{\mu}_{i}(t)^\complement$ and $E^{\theta}_{i}(t)^\complement$ the complementary event $E^{\mu}_{i}(t)$ and $E^{\theta}_{i}(t)$, respectively. Using Lemma~\ref{lemma:wald}, we can rewrite the regret as:
\begin{equation}
    R(\text{\texttt{$\gamma$-GTS}},T) \leq \sum_{i=2}^{K} {\Delta_{i}(T,0)} \E[N_{i,T}] =  \sum_{i=2}^{K} {\Delta_{i}(T,0)}\sum_{t=1}^{T}{\Prob(I_t=i)}.
\end{equation}
Let us focus on decomposing the probability term in the regret as follows:
\begin{align}
    \sum_{t=1}^{T}\Prob(I_t=i)  & =\underbrace{ \sum_{t=1}^{T} \Prob(I_t=i,E^{\mu}_{i}(t)^\complement)}_{=: P_A} + \underbrace{\sum_{t=1}^{T} \Prob(I_t=i,E^{\mu}_{i}(t),E^{\theta}_{i}(t)^\complement)}_{=: P_B} \\
    &  \quad + \underbrace{\sum_{t=1}^{T} \Prob(I_t = i, E^{\mu}_{i}(t), E^{\theta}_{i}(t))}_{=: P_C}.
\end{align}
The three terms correspond to the case of:
\begin{itemize}
    \item (i) having a poor estimation of the mean for arm $i$ (i.e., $P_A$);
    \item (ii) having a good estimation of the mean and having sampled a large value for the arm $i$ posterior sample (i.e., $P_B$);
    \item (iii) having a good estimate for the mean of the reward and having sampled a small value for the posterior sample of arm $i$ (i.e., $P_C$).
\end{itemize}
Let us analyze each term separately. We will neglect the error due to the round robin that will sum up to a constant w.r.t the time.

\paragraph{Term A}
Let $\tau_k \in \dsb{T}$ denote the round at which we pull the arm $i$ for the $k$-th time (we are omitting the dependence on the arm index $i$ to avoid heaving the notation).
In what follows, we let the sum run to times that can be greater than $T$.
We have:
\begin{align}
    P_A &= \sum_{t=K+1}^{T} \Prob(I_t =i, E^{\mu}_{i}(t)^\complement) \\
    & \leq \mathbb{E} \left[ \sum_{k=1}^{T} \sum_{t=\tau_k+1}^{\tau_{k+1}} \mathds{1} \left\{ I_t=i \right\} \mathds{1} \left\{ E^{\mu}_{i}(t)^\complement \right\} \right]\\
    & \leq \mathbb{E} \left[ \sum_{k=1}^{T-1} \mathds{1} \left\{ E^{\mu}_{i}(\tau_k+1)^\complement\right\} \underbrace{\sum_{t=\tau_k+1}^{\tau_{k+1}} \mathds{1} \left\{ I_t=i \right\}}_{= 1} \right]  \label{l:001} \\
    &  =\mathbb{E} \left[ \sum_{k=1}^{T-1} \mathds{1} \left\{ E^{\mu}_{i}(\tau_k+1)^\complement) \right\} \right]\\
    &\leq 1 + \mathbb{E} \left[ \sum_{k=1}^{T-1} \mathds{1} \left\{ E^{\mu}_{i}(\tau_k+1)^\complement \right\} \right] = 1 + \sum_{k=1}^{T-1} \underbrace{\Prob ( E^{\mu}_{i}(\tau_k+1)^\complement)}_{=:P_D},
\end{align}
where Equation~\eqref{l:001} follows from observing that the indicator function is $1$ in a single round in the inner summation.
Let us notice that thanks to the definition of the event $E^{\mu}_{i}(\tau_{k}+1)$, the term $P_D$ corresponds to the probability that $\overline{\hat{\mu}}_{i,\tau_k} > x_i$ after exactly $k$ pulls (which is not a random variable).
Thus, using Lemma~\ref{lemma:Subg} and recalling that $\E[\overline{\hat{\mu}}_{i,\tau_k} ]=\overline{\mu}_{i}(k)$, we have:
\begin{align}
    P_D & = \Prob ( \overline{\hat{\mu}}_{i,\tau_k}  > x_i) = \Prob(\overline{\hat{\mu}}_{i,\tau_k}  > \overline{\mu}_{i}(k) - \overline{\mu}_{i}(k) + x_i)\\
    & \leq \exp \left( -k\frac{(x_i-\overline{\mu}_i(k))^2}{2\sigma_{\textit{var}}^2} \right) \leq \exp \left( -k \frac{(x_i-\overline{\mu}_i(T))^2}{2\sigma_{\textit{var}}^2} \right),
\end{align}
This implies that:
\begin{equation}
    P_A \leq 1 + \sum_{k=1}^{T-1} \exp \left( -k\frac{(x_i-\overline{\mu}_i(T))^2}{2\sigma_{\textit{var}}^2} \right) \leq 1 + \frac{2\sigma_{\textit{var}}^2}{(x_i-\overline{\mu}_i(T))^2},
\end{equation}
where the last inequality follows by bounding the summation with the corresponding integral.

\paragraph{Term B}
Defining $L_i(T)=\frac{288\log(T\overline{\Delta}_i(\sigma_i,T)^2+e^{6})}{\gamma \overline{\Delta}_i(\sigma_i,T)^2}$, we decompose each summand into two parts:
\begin{align}
    P_B & = \sum_{t=K+1}^{T}\Prob\big(I_t=i,E^{\mu}_{i}(t),E^{\theta}_{i}(t)^\complement \big)\\
    &=\sum_{t=K+1}^{T}\Prob\big(I_t=i,k_i(t)\leq L_i(T), E^{\mu}_{i}(t),E^{\theta}_{i}(t)^\complement \big)+\Prob\big(I_t=i,k_i(t) >L_i(T), E^{\mu}_{i}(t),E^{\theta}_{i}(t)^\complement \big).
\end{align}
The first term is bounded by $L_i(T)$. For the second term:
\begin{align} \sum_{t=K+1}^T \Prob\left(i(t)=i, k_i(t)>L_i(T), E_i^\theta(t)^\complement, E_i^\mu(t)\right) & \leq \mathbb{E}\left[\sum_{t=K+1}^T \Prob\left(i(t)=i, {E_i^\theta(t)}^\complement \mid k_i(t)>L_i(T), E_i^\mu(t), \mathbb{F}_{t-1}\right)\right] \\ & \leq \mathbb{E}\left[\sum_{t=K+1}^T \Prob\left(\theta_i(t)>y_i \mid k_i(t)>L_i(T), \overline{\hat{\mu}}_i(t) \leq x_i, \mathbb{F}_{t-1}\right)\right].\end{align}
Now, $\theta_i(t)$ is a $\mathcal{N}\left(\overline{\hat{\mu}}_i(t), \frac{1}{\gamma k_i(t)}\right)$ distributed Gaussian random variable. An $\mathcal{N}\left(m, \sigma^2\right)$ distributed r.v. (i.e., a Gaussian random variable with mean $m$ and variance $\sigma^2$ ) is stochastically dominated by $\mathcal{N}\left(m^{\prime}, \sigma^2\right)$ distributed r.v. if $m^{\prime} \geq m$. Therefore, given $\overline{\hat{\mu}}_i(t) \leq x_i$, the distribution of $\theta_i(t)$ is stochastically dominated by $\mathcal{N}\left(\overline{\hat{\mu}}_i(t), \frac{1}{\gamma k_i(t)}\right)$. That is,
$$
\Prob\left(\theta_i(t)>y_i \mid k_i(t)>L_i(T), \overline{\hat{\mu}}_i(t) \leq x_i, \mathbb{F}_{t-1}\right) \leq \Prob\left(\left.\mathcal{N}\left(x_i, \frac{1}{\gamma k_i(t)}\right)>y_i \right\rvert\, \mathbb{F}_{t-1}, k_i(t)>L_i(T)\right).
$$

Here, we a slight abuse of notation we say that $\Prob\left(\mathcal{N}\left(m, \sigma^2\right)>y_i\right)$ represents the probability that a random variable distributed as $\mathcal{N}\left(m, \sigma^2\right)$ takes value greater than $y_i$. We have:
\begin{align}
    \Prob\left(\theta_i(t)>y_i \mid k_i(t)>L_i(T), \overline{\hat{\mu}}_i(t) \leq x_i, \mathbb{F}_{t-1}\right) \leq \Prob\left(\left.\mathcal{N}\left(x_i, \frac{1}{\gamma k_i(t)}\right)>y_i \right\rvert\, \mathbb{F}_{t-1}, k_i(t)>L_i(T)\right).
\end{align}
Using Lemma~\ref{lemma:Abramowitz2} we have:
\begin{align}
    \Prob\left(\mathcal{N}\left(x_i, \frac{1}{\gamma k_i(t)}\right)>y_i\right) & \leq \frac{1}{2} e^{-\frac{\left(\gamma k_i(t)\right)\left(y_i-x_i\right)^2}{2}} \\ & \leq \frac{1}{2} e^{-\frac{\left(\gamma L_i(T)\right)\left(y_i-x_i\right)^2}{2}},
\end{align}
which is smaller than $\frac{1}{T \overline{\Delta}_i(\sigma_i,T)^2}$ because $L_i(T) \geq \frac{2 \ln \left(T \overline{\Delta}_i(\sigma_i,T)^2\right)}{\gamma \left(y_i-x_i\right)^2}$. Substituting, we get,
\begin{equation}
   \Prob\left(\theta_i(t)>y_i \mid k_i(t)>L_i(T), \hat{\mu}_i(t) \leq x_i, \mathcal{F}_{t-1}\right) \leq \frac{1}{T\overline{\Delta}_i(\sigma_i,T)^2}. 
\end{equation}

Summing over $t=1, \ldots, T$, we get a bound of $\frac{1}{\overline{\Delta}_i(\sigma_i,T)^2}$.
\paragraph{Term C}
For this term, we shall use Lemma~1 by~\cite{agrawal2017near}. Let us define $p_{i,t} = \Prob(\theta_{1,t} > y_i | \mathbb{F}_{t-1})$. We have:
\begin{equation}
    \Prob(I_t = i, E^{\mu}_{i}(t), E^{\theta}_{i}(t) | \mathbb{F}_{t-1}) \leq \frac{1-p_{i,t}}{p_{i,t}} \Prob(I_t = 1, E^{\mu}_{i}(t), E^{\theta}_{i}(t)|\mathbb{F}_{t-1}).
\end{equation}
Thus, we can rewrite the term $P_C$ as follows:
\begin{align}
    P_C  & = \sum_{t=K+1}^{T}\Prob(I_t=i,E^{\mu}_{i}(t),E^{\theta}_{i}(t)) \\
    & = \sum_{t=K+1}^{T} \mathbb{E}[\Prob(I_t=i,E^{\mu}_{i}(t),E^{\theta}_{i}(t)|\mathbb{F}_{t-1})] \\
    &\leq \sum_{t=K+1}^{T}\mathbb{E}\bigg[\mathbb{E}\bigg[\frac{1-p_{i,t}}{p_{i,t}}\mathds{1}(I_t=1,E^{\mu}_{i}(t),E^{\theta}_{i}(t))\bigg|\mathbb{F}_{t-1}\bigg]\bigg] \\
    &\leq\sum_{t=K+1}^{T}\mathbb{E}\bigg[\frac{1-p_{i,t}}{p_{i,t}}\mathds{1}(I_t=1,E^{\mu}_{i}(t),E^{\theta}_{i}(t))\bigg].\\
\end{align}
Let $\tau_k$ denote the time step at which arm $1$ is played for the $k$-th time (notice we allow the sum to run trough times bigger than the learning horizon $T$), and let $\tau_0 = 0$:
\begin{align}
    P_C &\leq \sum_{k=1}^{T-1}\mathbb{E}\bigg[\frac{1-p_{i,\tau_{k}+1}}{p_{i,\tau_{k}+1}}\sum_{t=\tau_k+1}^{\tau_{k+1}}\mathds{1}(I_t=1,E^{\mu}_{i}(t),E^{\theta}_{i}(t))\bigg]\\
    &\leq\sum_{k=1}^{T-1}\mathbb{E}\bigg[\frac{1-p_{i,\tau_k+1}}{p_{i,\tau_k+1}}\bigg], \label{eq:fixed2}
\end{align}
where the inequality in Equation~\eqref{eq:fixed2} uses the fact that $p_{i,t}$ is fixed, given $\mathbb{F}_{t-1}$. Then, we observe that $p_{i,t} = \Prob(\theta_{1,t} > y_i |\mathbb{F}_{t-1})$
changes only when the distribution of $\theta_{1,t}$ changes, that is, only on the time step after each play of the first arm. Thus, $p_{i,t}$ is the same at all time steps $t \in \{\tau_k+1, \dots , \tau_{k+1}\}$, for every $k$. Finally, bounding the probability of selecting the optimal arm by $1$ we have:
\begin{equation}
    P_C \leq \sum_{k=1}^{T-1}\mathbb{E} \left[ \frac{1}{p_{i,\tau_k+1}} - 1 \right].
\end{equation}
Now in order to face this term, let's consider the arbitrary $j-th$ trial, $\forall$ $j$ thanks to Lemma \ref{lemma:changeMeasure} we can bound the difference between the real process and an analogous (same number of trials) virtual process with mean $\overline{\mu}_1(\sigma_i)$ (where by stationary we mean that all the trials of the virtual process will have a fixed mean):
\begin{align}
    \underbrace{\mathbb{E}_{\overline{\mu}_1(j)} \left[ \frac{1}{p_{i,\tau_j+1}}  \right]}_{(*)} \leq \frac{2\delta_{TV}(\mathbb{P}_j,\mathbb{Q}_j(\overline{\mu}_{1}(\sigma_i)))}{\textbf{erfc}(\sqrt{\frac{\gamma j}{2}}\overline{\mu}_1(\sigma_i))}+\underbrace{\mathbb{E}_{\overline{\mu}_1(\sigma_i)} \left[ \frac{1}{p_{i,\tau_j+1}} \right]}_{(**)}. 
\end{align}
where $\delta_{TV}(P,Q) \coloneqq \sup_{A\in\mathcal{F}}{\big|P(A)-Q(A)\big|}$ is the total variation between the probability measures $P$ and $Q$ (assuming they are defined over a measurable space $(\Omega,\mathcal{F})$, having observed that, using the notation of Lemma~\ref{lemma:changeMeasure} (as the environment can't produce rewards smaller than zero):
\begin{align}
    & b= \max_{s} \frac{1}{\Prob\left(\mathcal{N}\left(s, \frac{1}{\gamma k_i(t)}\right)>y_i\right)} \leq\frac{1}{\Prob\left(\mathcal{N}\left(0, \frac{1}{\gamma k_i(t)}\right)\ge \overline{\mu}_1(\sigma_i)\right)} =  \frac{2}{\textbf{erfc}(\sqrt{\frac{\gamma j}{2}}\overline{\mu}_1(\sigma_i))}, \\
    & a= 1.  
\end{align}
For example, as both binomial and poisson-binomial process are subgaussian, when we have a poisson-binomial process the analogous one shall be a binomial with fixed mean,  $\overline{\mu}_1(\sigma_i)$ and $\sigma_{\textit{var}}^2$ will be $\frac{1}{4}$, in general for bounded random variables between $[a,b]$, i.e the samples can be sampled only within $[a,b]$, we will have in what follows $\sigma_{\textit{var}}^2=\frac{(b-a)^2}{4}$, then for this process the analogous will be a stationary process in which the samples can be sampled within interval $[a,b]$ centered in $\overline{\mu}_1(\sigma_i)$ considered for the same number of trials (like for the example can be the sum of uniform random variables). When the interval changes at every trials, without loss of generality in what follows we can take $\sigma_{\textit{var}}^2$ as the maximum of these variances, i.e. the maximum variance a sample can have in the setting. For random variables explicitly written in term of a mean and a variance term (like the Gaussian) holds the same. Our interest is to find if there is a minimum number of trials $j$ such that we will have $(*)\ge(**)$ without any adding term.
Given $\mathbb{F}_{\tau_j}$, let $\Theta_j$ denote a $\mathcal{N}\left(\overline{\hat{\mu}}_1\left(\tau_j+1\right), \frac{1}{\gamma j}\right)$ distributed Gaussian random variable. Let $G_j$ be the geometric random variable denoting the number of consecutive independent trials until and including the trial where a sample of $\Theta_j$ becomes greater than $y_i$. Then observe that $p_{i, \tau_j+1}=\operatorname{Pr}\left(\Theta_j>y_i \mid \mathbb{F}_{\tau_j}\right)$ and
\begin{align}\label{eq:rif}
    \mathbb{E}\left[\frac{1}{p_{i, \tau_j+1}}\right]=\mathbb{E}\left[\mathbb{E}\left[G_j \mid \mathbb{F}_{\tau_j}\right]\big]=\mathbb{E}\left[G_j\right]\right.
\end{align}

We compute first the expected value for the real process. We will consider first $j$ such that $\overline{\mu}_1(j)\ge \overline{\mu}_1(\sigma_i)$ , we will bound the expected value of $G_j$ by a constant for all $j$ defined as earlier.
Consider any integer $r \geq 1$. Let $z=\sqrt{\ln r}$ and let random variable MAX $_r$ denote the maximum of $r$ independent samples of $\Theta_j$. We abbreviate $\overline{\hat{\mu}}_1\left(\tau_j+1\right)$ to $\overline{\hat{\mu}}_1$ and we will abbreviate $\overline{\mu}_1(j)$ as $\mu_1$ and $\overline{\Delta}_i(j,T)$ as $\Delta_i$ in the following. Then for any integer $r\ge 1$:
\begin{align} \Prob\left(G_j \leq r\right) & \geq \Prob\left(\operatorname{MAX}_r>y_i\right) \\ & \geq \Prob\left(\operatorname{MAX}_r>\overline{\hat{\mu}}_1+\frac{z}{\sqrt{\gamma j}} \geq y_i\right) \\ & =\mathbb{E}\left[\mathbb{E}\left[\left.\mathds{1}\left(\operatorname{MAX}_r>\overline{\hat{\mu}}_1+\frac{z}{\sqrt{\gamma j}} \geq y_i\right) \right\rvert\, \mathbb{F}_{\tau_j}\right]\right] \\ & =\mathbb{E}\left[\mathds{1}\left(\overline{\hat{\mu}}_1+\frac{z}{\sqrt{\gamma j}} \geq y_i\right) \Prob\left(\left.\operatorname{MAX}_r>\overline{\hat{\mu}}_1+\frac{z}{\sqrt{\gamma j}} \right\rvert\, \mathbb{F}_{\tau_j}\right)\right]\end{align}
For any instantiation $F_{\tau_j}$ of $\mathbb{F}_{\tau_j}$, since $\Theta_j$ is Gaussian $\mathcal{N}\left(\hat{\mu}_1, \frac{1}{\gamma j}\right)$ distributed r.v., this gives using \ref{lemma:Abramowitz}:
\begin{align}
    \Prob\left(\left.\operatorname{MAX}_r>\overline{\hat{\mu}}_1+\frac{z}{\sqrt{\gamma j}} \right\rvert\, \mathbb{F}_{\tau_j}=F_{\tau_j}\right) & \geq 1-\left(1-\frac{1}{\sqrt{2 \pi}} \frac{z}{\left(z^2+1\right)} e^{-z^2 / 2}\right)^r \\ & =1-\left(1-\frac{1}{\sqrt{2 \pi}} \frac{\sqrt{\ln r}}{(\ln r+1)} \frac{1}{\sqrt{r}}\right)^r \\ & \geq 1-e^{-\frac{r}{\sqrt{4 \pi r \ln r}}}.
\end{align}
For $r \ge e^{12}$:
\begin{align}
   \Prob\left(\left.\operatorname{MAX}_r>\overline{\hat{\mu}}_1+\frac{z}{\sqrt{\gamma j}} \right\rvert\, \mathbb{F}_{\tau_j}=F_{\tau_j}\right) \geq 1-\frac{1}{r^2}. 
\end{align}
Substituting we obtain:
\begin{align}
    \Prob\left(G_j \leq r\right) & \geq \mathbb{E}\left[\mathds{1}\left(\overline{\hat{\mu}}_1+\frac{z}{\sqrt{\gamma j}} \geq y_i\right)\left(1-\frac{1}{r^2}\right)\right] \\ & =\left(1-\frac{1}{r^2}\right) \Prob\left(\overline{\hat{\mu}}_1+\frac{z}{\sqrt{\gamma j}} \geq y_i\right).
\end{align}
Applying Lemma~\ref{lemma:Subg} to the second term, we can write:
\begin{align}
  \Prob\left(\overline{\hat{\mu}}_1+\frac{z}{\sqrt{\gamma j}} \geq \mu_1\right) \geq 1-e^{-\frac{z^2}{2\gamma \sigma_{\textit{var}}^2}} \geq 1-\frac{1}{r^2},  
\end{align}
being $\gamma\leq \frac{1}{4\sigma_{\textit{var}}^2}$. Using, $y_i \leq \mu_1$, this gives
\begin{equation}
   \Prob\left(\overline{\hat{\mu}}_1+\frac{z}{\sqrt{\gamma j}} \geq y_i\right) \geq 1-\frac{1}{r^2} . 
\end{equation}
Substituting all back we obtain:
\begin{align}
    \mathbb{E}\left[G_j\right] & =\sum_{r=0}^{\infty} \Prob\left(G_j \geq r\right) \\ & =1+\sum_{r=1}^{\infty} \Prob\left(G_j \geq r\right) \\ & \leq 1+e^{12}+\sum_{r \geq 1}\left(\frac{1}{r^2}+\frac{1}{r^{2}}\right) \\ & \leq 1+e^{12}+2+2.
\end{align}
This shows a constant bound of $\mathbb{E}\left[\frac{1}{p_{i, \tau_j+1}}-1\right]=\mathbb{E}\left[G_j\right]-1 \leq e^{12}+5$ for all $j\ge \sigma_i$.
We derive a  bound for large $j$. Consider $j>L_i(T)$ (and still $j\ge\sigma_i$). Given any $r \geq 1$, define $G_j, \operatorname{MAX}_r$, and $z=\sqrt{\ln r}$ as defined earlier. Then,
\begin{align} \Prob\left(G_j \leq r\right) & \geq \Prob\left(\operatorname{MAX}_r>y_i\right) \\ & \geq \Prob\left(\operatorname{MAX}_r>\overline{\hat{\mu}}_1+\frac{z}{\sqrt{\gamma j}}-\frac{\Delta_i}{6} \geq y_i\right) \\ & =\mathbb{E}\left[\mathbb{E}\left[\left.\mathds{1}\left(\operatorname{MAX}_r>\overline{\hat{\mu}}_1+\frac{z}{\sqrt{\gamma j}}-\frac{\Delta_i}{6} \geq y_i\right) \right\rvert\, \mathbb{F}_{\tau_j}\right]\right] \\ & =\mathbb{E}\left[\mathds{1}\left(\overline{\hat{\mu}}_1+\frac{z}{\sqrt{\gamma j}}+\frac{\Delta_i}{6} \geq \mu_1\right) \Prob\left(\left.\operatorname{MAX}_r>\overline{\hat{\mu}}_1+\frac{z}{\sqrt{\gamma j}}-\frac{\Delta_i}{6} \right\rvert\, \mathbb{F}_{\tau_j}\right)\right] .\end{align}
where we used that $y_i=\mu_1-\frac{\Delta_i}{3}$. Now, since $j \geq L_i(T)=\frac{288 \ln \left(T \Delta_i^2+e^{6}\right)}{\gamma\Delta_i^2}$,
\begin{align}
    2 \frac{\sqrt{2 \ln \left(T \Delta_i^2+e^{6}\right)}}{\sqrt{\gamma j}} \leq \frac{\Delta_i}{6}.
\end{align}

Therefore, for $r \leq\left(T \Delta_i^2+e^{6}\right)^2$,
\begin{align}
 \frac{z}{\sqrt{\gamma j}}-\frac{\Delta_i}{6}=\frac{\sqrt{\ln (r)}}{\sqrt{\gamma j}}-\frac{\Delta_i}{6} \leq-\frac{\Delta_i}{12}.
\end{align}

Then, since $\Theta_j$ is $\mathcal{N}\left(\overline{\hat{\mu}}_1\left(\tau_j+1\right), \frac{1}{\gamma j}\right)$ distributed random variable, using the upper bound in Lemma \ref{lemma:Abramowitz2}, we obtain for any instantiation $F_{\tau_j}$ of history $\mathbb{F}_{\tau_j}$,
\begin{align}
    \Prob\left(\left.\Theta_j>\overline{\hat{\mu}}_1\left(\tau_j+1\right)-\frac{\Delta_i}{12} \right\rvert\, \mathbb{F}_{\tau_j}=F_{\tau_j}\right) \geq 1-\frac{1}{2} e^{-\gamma j \frac{\Delta_i^2}{288}} \geq 1-\frac{1}{2\left(T \Delta_i^2+e^{6}\right)}.
\end{align}
being $j\geq L_i(T)$. This implies:
\begin{align}
    \Prob\left(\left.\operatorname{MAX}_r>\hat{\mu}_1\left(\tau_j+1\right)+\frac{z}{\sqrt{\gamma j}}-\frac{\Delta_i}{6} \right\rvert\, \mathbb{F}_{\tau_j}=F_{\tau_j}\right) \geq 1-\frac{1}{2^r\left(T \Delta_i^2+e^{6}\right)^r}.
\end{align}

Also, for any $t \geq \tau_j+1$, we have $k_1(t) \geq j$, and using Lemma~\ref{lemma:Subg}, we get:
\begin{align}
\Prob\left(\overline{\hat{\mu}}_1(t)+\frac{z}{\sqrt{\gamma j}}-\frac{\Delta_i}{6} \geq y_i\right) \geq \Prob\left(\overline{\hat{\mu}}_1(t) \geq \mu_1-\frac{\Delta_i}{6}\right) \geq 1-e^{- k_1(t) \Delta_i^2 / 72\sigma^2_{\textit{var}}} \geq 1-\frac{1}{\left(T \Delta_i^2+e^{6}\right)^{16}}.
\end{align}

Let $T^{\prime}=\left(T \Delta_i^2+e^{6}\right)^2$. Therefore, for $1 \leq r \leq T^{\prime}$, we have:
\begin{align}
    \Prob\left(G_j \leq r\right) \geq 1-\frac{1}{2^r\left(T^{\prime}\right)^{r / 2}}-\frac{1}{\left(T^{\prime}\right)^8}.
\end{align}

When $r \geq T^{\prime} \geq e^{12}$, we obtain:
\begin{align}
    \Prob\left(G_j \leq r\right) \geq 1-\frac{1}{r^2}-\frac{1}{r^{2}}.
\end{align}

Combining all the bounds we have derived:
    \begin{align} \mathbb{E}\left[G_j\right] & \leq \sum_{r=0}^{\infty} \Prob\left(G_j \geq r\right) \\ & \leq 1+\sum_{r=1}^{T^{\prime}} \Prob\left(G_j \geq r\right)+\sum_{r=T^{\prime}}^{\infty} \Prob\left(G_j \geq r\right) \\ & \leq 1+\sum_{r=1}^{T^{\prime}} \frac{1}{\left(2 \sqrt{T^{\prime}}\right)^r}+\frac{1}{\left(T^{\prime}\right)^7}+\sum_{r=T^{\prime}}^{\infty} \frac{1}{r^2}+\frac{1}{r^{1.5}} \\ & \leq 1+\frac{1}{\sqrt{T^{\prime}}}+\frac{1}{\left(T^{\prime}\right)^7}+\frac{2}{T^{\prime}}+\frac{3}{\sqrt{T^{\prime}}} \\ & \leq 1+\frac{5}{T \Delta_i^2+e^{6}} .\end{align}

So we have proved that:
\begin{align}
    \mathbb{E}\left[\frac{1}{p_{i, \tau_j+1}}\right]\le\begin{cases}
                 \frac{2\delta_{TV}(\mathbb{P}_j(\overline{\mu}_{1}(j)),\mathbb{P}_j(\overline{\mu}_{1}(\sigma_i)))}{\textbf{erfc}(\sqrt{\frac{\gamma j}{2}}\overline{\mu}_1(\sigma_i))}+\mathbb{E}_{\overline{\mu}_1(\sigma_i)} \left[ \frac{1}{p_{i,\tau_j+1}} \right].  & \text{if } 0 \le j<\sigma_i \\
                %\Big(\frac{1}{(1-y_i)^{j+1}}-1\Big)\delta_{\text{TV}}(\text{PB}(\underline{\mu}_{1}(j)),\text{Bin}(j,\overline{\mu}_{1}(j)))+ \sum_{s=0}^{j} \frac{f_{j,\overline{\mu}_{1}(\sigma_i)}(s)}{F_{j+1, y_i^B}(s)} & \text{if } \sigma_i \le j<\xi_i \\
                (e^{12}+5) & \text{if } j\ge\sigma_i \\
                \frac{5}{T\overline{\Delta}_i(j,T)^2} &\textit{if } j\ge L_i(T,j) \textit{ and } j\ge\sigma_i 
        \end{cases}
\end{align}
Notice that $L_i(T,j)=\frac{288\log(T\overline{\Delta}_i(j,T)^2+e^6)}{\gamma\overline{\Delta}_i^2(j,T)}$ is decreasing w.r.t.~$\overline{\Delta}_i(j,T)$, so we can write:

\begin{align}
    \mathbb{E}\left[\frac{1}{p_{i, \tau_j+1}}\right]\le\begin{cases}
                 \frac{2\delta_{TV}(\mathbb{P}_j(\overline{\mu}_{1}(j)),\mathbb{P}_j(\overline{\mu}_{1}(\sigma_i)))}{\textbf{erfc}(\sqrt{\frac{\gamma j}{2}}\overline{\mu}_1(\sigma_i))}+\mathbb{E}_{\overline{\mu}_1(\sigma_i)} \left[ \frac{1}{p_{i,\tau_j+1}} \right].  & \text{if } 0 \le j<\sigma_i \\
                %\Big(\frac{1}{(1-y_i)^{j+1}}-1\Big)\delta_{\text{TV}}(\text{PB}(\underline{\mu}_{1}(j)),\text{Bin}(j,\overline{\mu}_{1}(j)))+ \sum_{s=0}^{j} \frac{f_{j,\overline{\mu}_{1}(\sigma_i)}(s)}{F_{j+1, y_i^B}(s)} & \text{if } \sigma_i \le j<\xi_i \\
                (e^{12}+5) & \text{if } j\ge\sigma_i \\
                \frac{5}{T\overline{\Delta}_i(j,T)^2} &\textit{if } j\ge \frac{288\log(T\overline{\Delta}_i^2(\sigma_i,T)+e^6)}{\gamma\overline{\Delta}_i^2(j,T)} \textit{ and } j\ge\sigma_i
        \end{cases}
\end{align}
By definition, we have:
\begin{align}
    \mathbb{E}\left[\frac{1}{p_{i, \tau_j+1}}\right]\le\begin{cases}
                 \frac{2\delta_{TV}(\mathbb{P}_j(\overline{\mu}_{1}(j)),\mathbb{P}_j(\overline{\mu}_{1}(\sigma_i)))}{\textbf{erfc}(\sqrt{\frac{\gamma j}{2}}\overline{\mu}_1(\sigma_i))}+\mathbb{E}_{\overline{\mu}_1(\sigma_i)} \left[ \frac{1}{p_{i,\tau_j+1}} \right].  & \text{if } 0 \le j<\sigma_i \\
                %\Big(\frac{1}{(1-y_i)^{j+1}}-1\Big)\delta_{\text{TV}}(\text{PB}(\underline{\mu}_{1}(j)),\text{Bin}(j,\overline{\mu}_{1}(j)))+ \sum_{s=0}^{j} \frac{f_{j,\overline{\mu}_{1}(\sigma_i)}(s)}{F_{j+1, y_i^B}(s)} & \text{if } \sigma_i \le j<\xi_i \\
                (e^{12}+5) & \text{if } j\ge\sigma_i \\
                \frac{5}{T\overline{\Delta}_i(\sigma_i,T)^2} &\textit{if } j\ge \frac{288\log(T\overline{\Delta}_i^2(\sigma_i,T)+e^6)}{\gamma\overline{\Delta}_i^2(\sigma_i,T)} \textit{ and } j\ge\sigma_i
        \end{cases}
\end{align}
We can end up in two scenarios:
\paragraph{First Case}
It may happen that $\sigma_i\ge \frac{288\log(T\overline{\Delta}_i^2(\sigma_i,T)+e^6)}{\gamma\overline{\Delta}_i^2(\sigma_i,T)}$, then, in this case, we already are in a situation in which we will sum $T-\sigma_i$ times the term $\frac{5}{T\overline{\Delta}_i(\sigma_i,T)^2}$.

\paragraph{Second Case}
The second case is the scenario in which we have $\sigma_i\leq\frac{288\log(T\overline{\Delta}_i^2(\sigma_i,T)+e^6)}{\gamma\overline{\Delta}_i^2(\sigma_i,T)}$.
In this situation we will sum $\frac{288\log(T\overline{\Delta}_i^2(\sigma_i,T)+e^6)}{\gamma\overline{\Delta}_i^2(\sigma_i,T)}-\sigma_i$ times the constant bound $(e^{12}+5)$ and $T-\frac{288\log(T\overline{\Delta}_i^2(\sigma_i,T)+e^6)}{\gamma\overline{\Delta}_i^2(\sigma_i,T)}$ times the term $\frac{5}{T\overline{\Delta}_i(\sigma_i,T)^2}$.

Notice that what we have found is the same bound we would  find doing the exact same passages for $\mathbb{E}_{\overline{\mu}_1(\sigma_i)} \left[ \frac{1}{p_{i,\tau_j+1}} \right]$ for $j\ge\sigma_i$, furthermore the inequality for $\mathbb{E}_{\overline{\mu}_1(\sigma_i)} \left[ \frac{1}{p_{i,\tau_j+1}} \right]$ holds true for any j by definition, i.e. it's easy to show that:
\begin{align}
  \mathbb{E}_{\overline{\mu}_1(\sigma_i)} \left[ \frac{1}{p_{i,\tau_j+1}} \right] \leq 
  \begin{cases}
      (e^{12}+5) &\textit{ } \forall j \\
      \frac{1}{T\overline{\Delta}_i(\sigma_i)^2} &\textit{if } j\ge \frac{288\log(T\overline{\Delta}_i^2(\sigma_i,T)+e^6)}{\gamma\overline{\Delta}_i^2(\sigma_i,T)}
  \end{cases}  
\end{align}
So that summing all the terms:

\begin{align}
    P_C \leq \sum_{k=0}^{T-1}\mathbb{E} \left[ \frac{1}{p_{i,\tau_k+1}} - 1 \right]\leq (e^{12}+5)\frac{288\log(T\overline{\Delta}_i^2(\sigma_i,T)+e^6)}{\gamma\overline{\Delta}_i^2(\sigma_i,T)}+ \nonumber \\
    +\frac{5}{\overline{\Delta}_i^2(\sigma_i,T)}+\sum_{j=1}^{{\sigma}-1}\frac{2\delta_{\text{TV}}(\mathbb{P}_j(\overline{\mu}_{1}(j)),\mathbb{P}_j(\overline{\mu}_{1}(\sigma)) }{\textbf{erfc}(\sqrt{\frac{{\gamma j}}{2}}(\overline{\mu}_1(\sigma)))}. 
\end{align}
By choosing $\sigma_i=\sigma$ and summing all the other term follows the statement. Notice furthermore that as a corollary we've proven in this way the optimality of \texttt{$\gamma$-GTS} for the generic subgaussian stationary environment.
\end{proof}}
\gtscor*
\begin{proof}
   If the arms' dynamics is such that exists a finite time horizon $T^*$ defined as:
\begin{align}
\overline{\mu}_1(T^*)>\overline{\mu}_i(+\mathcal{1}),\text{ } \forall i \neq 1,
\end{align}
i.e., informally, there's a finite time over which the best arm won't change anymore, we can devise a finite grid of values for every $T$ and every $i$ of $\overline{\Delta}_i(\sigma(T),T)$ (we have taken $\sigma(T)$ for the sake if the argument, notice however that for every $T$ we could choose any $\sigma\in \dsb{\sigma(T),T}$) up to $T^*$, for $T^*$ we will consider $\overline{\Delta}_i(T^*,\mathcal{1})$. Then it is possible to define a constant $c$ as in \ref{eq:costante}. In fact notice that for all $T\ge T^*$, taking in what we've proved earlier $\sigma=T^*$ for every time horizon $T\ge T^*$, the sum of the total variation distances becomes a constant with respect to the time and substituting in all the terms for $T\ge T^*$, $\Delta_i{(T^*,T)}$ with $\Delta_i{(T^*,\mathcal{1})}$, we obtain (neglecting the constant terms with respect to the time), since all the terms are increasing for decreasing  $\overline{\Delta}_i(\sigma(T),T)$, we find:
\begin{align}
  R(\text{\texttt{$\gamma$-GTS}},T)\leq O \Bigg( \sum_{i=2}^K \Delta_i(T,0)\Big(C_1\frac{\log (T\overline{\Delta}_i(T^*,T)^2+e^{6})}{\gamma\overline{\Delta}_i(T^*,T)^2}
     +\frac{18\sigma^2_{\textit{var}}+6}{\overline{\Delta}_i(T^*,T)^2}\Big) \Bigg), 
\end{align}
Then, by definition:
\begin{align}
     R(\text{\texttt{$\gamma$-GTS}},T)\leq O \Bigg( \sum_{i=2}^K \Delta_i(T,0)\Big(C_1\frac{\log (T\overline{\Delta}_i(T^*,\mathcal{1})^2+e^{6})}{\gamma\overline{\Delta}_i(T^*,\mathcal{1})^2}
     +\frac{18\sigma^2_{\textit{var}}+6}{\overline{\Delta}_i(T^*,\mathcal{1})^2}\Big) \Bigg).
\end{align}

Notice that also the second term in the above inequality is time-independent for $T \ge T^*$.
Using the definition of $c$ (Equation~\eqref{eq:costante}), we can rewrite the regret as follows:
\begin{equation}
     R(\text{\texttt{$\gamma$-GTS}},T)\leq O \Bigg( \sum_{i=2}^K c\Delta_i(\sigma(T^*),\mathcal{1})\Big(C_1\frac{\log (T\overline{\Delta}_i(T^*,\mathcal{1})^2+e^{6})}{\gamma\overline{\Delta}_i(T^*,\mathcal{1})^2}\Big) \Bigg).
\end{equation}
Disregarding the constant terms w.r.t.~time $T$:
\begin{equation}
    R(\text{\texttt{$\gamma$-GTS}},T)\leq O \Bigg( \sum_{i=2}^K \Delta_i(T^*,\mathcal{1})\Big(\frac{\log (T\overline{\Delta}_i(T^*,\mathcal{1})^2+e^{6})}{\overline{\Delta}_i(T^*,\mathcal{1})^2}\Big) \Bigg),
\end{equation}
that is equivalent to the bound provided for the classical instance-independent regret bound by~\cite{agrawal2012analysis} for the stationary sunbgaussian bandit.

Now consider $T\leq T^*$, we can write, using the definition of $c$ in Equation~\eqref{eq:cdefin}:
\begin{align}
     R(\text{\texttt{$\gamma$-GTS}},T)\leq O \Bigg( \sum_{i=2}^K c\overline{\Delta}_i(\sigma(T),T)\Big(C_1\frac{\log (T\overline{\Delta}_i(\sigma(T),\mathcal{1})^2+e^{6})}{\gamma\overline{\Delta}_i(\sigma(T),T)^2}+\nonumber \\
     +\frac{18\sigma^2_{\textit{var}}+6}{\overline{\Delta}_i(\sigma(T),T)^2} + \sum_{j=1}^{{\sigma(T)}-1}\frac{2\delta_{\text{TV}}(\mathbb{P}_j,\mathbb{Q}_j(\overline{\mu}_{1}(\sigma(T))) }{\textbf{erfc}(\sqrt{\frac{{\gamma j}}{2}}(\overline{\mu}_1(\sigma(T))))}  \Big)  \Bigg), 
\end{align}
We notice that thanks to the definition of $c$ in \ref{eq:costante}, $\frac{18\sigma^2_{\textit{var}}+6}{\overline{\Delta}_i(\sigma(T),T)^2} $ is bounded with a constant term with respect to the time horizon $T$. Then, we have:
\begin{align}
  R(\text{\texttt{$\gamma$-GTS}},T)\leq O \Bigg( \sum_{i=2}^K c\overline{\Delta}_i(\sigma(T),T)\Big(C_1\frac{\log (T\overline{\Delta}_i(\sigma(T),\mathcal{1})^2+e^{6})}{\gamma\overline{\Delta}_i(\sigma(T),T)^2}
     + \sum_{j=1}^{{\sigma(T)}-1}\frac{2\delta_{\text{TV}}(\mathbb{P}_j,\mathbb{Q}_j(\overline{\mu}_{1}(\sigma(T))) }{\textbf{erfc}(\sqrt{\frac{{\gamma j}}{2}}(\overline{\mu}_1(\sigma(T))))}  \Big)  \Bigg),   
\end{align}
\cite{chang2011cerf} proved that the complementary error function che be bounded lower-bounded as:
\begin{equation}
    \textbf{ercf}(x)\geq \sqrt{\frac{ e}{\pi}}  e^{-2 x^2}
\end{equation}
so by loosely bounding the total variation distances with $1$ and recognising the geometric series we get:
\begin{align}
  R(\text{\texttt{$\gamma$-GTS}},T)\leq O \Bigg( \sum_{i=2}^K c\overline{\Delta}_i(\sigma(T),T)\Big(C_1\frac{\log (T\overline{\Delta}_i(\sigma(T),T)^2+e^{6})}{\gamma\overline{\Delta}_i(\sigma(T),T)^2}
     + C_2 e^{\gamma\sigma(T)\overline{\mu}_1(\sigma(T))^2} \Big)  \Bigg),   
\end{align}
so that:
\begin{align}
  R(\text{\texttt{$\gamma$-GTS}},T)\leq O \Bigg( \sum_{i=2}^K c\overline{\Delta}_i(\sigma(T),T)\Big(\frac{\log (T\overline{\Delta}_i(\sigma(T),T)^2+e^6)}{\gamma\overline{\Delta}_i(\sigma(T),T)^2} +e^{\gamma\sigma(T)\overline{\mu}_1(\sigma(T))^2}\Big)  \Bigg),  \label{eq:cases}
\end{align}
considering then the two cases:
\begin{align}
    \overline{\Delta}_i(\sigma(T),T)&\leq e\sqrt{K\frac{1}{\gamma T}},\\
    \overline{\Delta}_i(\sigma(T),T)&\ge e\sqrt{K\frac{1}{\gamma T}}.
\end{align}
Substituting the above cases in Equation~\eqref{eq:cases}, concludes the proof.
\end{proof}

\gammagts*
\begin{proof}
   The proof follows from the proof of the previous theorem setting $\gamma=T^{-\alpha}$, with $\alpha$ within the bounds given in the statement of the theorem.
\end{proof}

\clearpage
\section{Proofs of Section~\ref{sec:SWapproach}}
In this section, we report the proof of the sliding window approach version of the algorithms we proposed. We also present the pseudocode for the \texttt{Beta-SWTS} and \texttt{$\gamma$-SWGTS} algorithms in Algorithm~\ref{alg:swbetats} and~\ref{alg:swgts}, respectively.

\begin{figure}[t]
\begin{minipage}{.43\textwidth}
\begin{algorithm}[H]
\caption{\texttt{Beta-SWTS} Algorithm} \label{alg:swbetats}
\small
\begin{algorithmic}[1]
    \STATE \textbf{Input:} Number of arms $K$, Time horizon $T$, time window $\tau$
    \STATE Set $\hat{\mu}_{i,1,\tau} \gets 0$ for each $i \in \dsb{K}$
    \STATE Set $\alpha_{i,1}\gets 1+ \hat{\mu}_{i,1,\tau}$ and $\beta_{i,1}\gets 1+ (1-\hat{\mu}_{i,1,\tau})$ for each $i \in \dsb{K}$
    \STATE Set $\nu_{i,1} \gets Beta(\alpha_{i,1}, \beta_{i,1})$ for each $i \in \dsb{K}$ \label{line:beta2}
    \FOR{$t \in \dsb{T}$}
        \STATE Sample $\theta_{i,t,\tau} \sim \nu_{i,t}$ for each $i \in \dsb{K}$ \label{line:sample2}
        \STATE Select $I_t \in \arg \max_{i \in \dsb{K}} \theta_{i,t,\tau}$ \label{line:selectionts2}
        \STATE Pull arm $I_t$
        \STATE Collect reward $X_t$
        \STATE Update $\hat{\mu}_{i,t,\tau}$ and $T_{i,t,\tau}$, respectively the sum of collected rewards within $t$ and $t-\tau+1$ for arm $i$ and the number arm $i$ has been pulled within $t$ and $t-\tau+1$
        \STATE Update for each $i \in \dsb{K}$ $\nu_{i,t+1} \gets \text{Beta}(1+\hat{\mu}_{i,t,\tau},1+(T_{i,t,\tau}-\hat{\mu}_{i,t,\tau}))$ \label{line:updatets2}
    \ENDFOR
\end{algorithmic}
\end{algorithm}
\end{minipage}\hfill
\begin{minipage}{.55\textwidth}
\begin{algorithm}[H]
\caption{\texttt{$\gamma$-SWGTS} Algorithm} \label{alg:swgts}
\small
\begin{algorithmic}[1]
    \STATE \textbf{Input:} Number of arms $K$, Time horizon $T$, exploration parameter $\gamma$, time window $\tau$
    \STATE Play every arm once and collect reward $X_t$
    \STATE Set $T_{i,t,\tau} \gets 1$,  $\hat{\mu}_{i,t,\tau} \gets X_t$, $\overline{\hat{\mu}}_{i,t,\tau} \gets \hat{\mu}_{i,t,\tau}$  for each $i \in \dsb{K}$
    \STATE Set $\nu_{i,t} \gets \mathcal{N}(\overline{\hat{\mu}}_{i,t,\tau},\frac{1}{\gamma})$ for each $i \in \dsb{K}$ \label{line:prior1}
    \FOR{$t \in \dsb{T}$}
        \STATE Sample $\theta_{i,t, \tau} \sim \nu_{i,t}$ for each $i \in \dsb{K}$ \label{line:sample11}
        \STATE Select $I_t \in \arg \max_{i \in \dsb{K}} \theta_{i,t,\tau}$ \label{line:selectionts11}
        \STATE Pull arm $I_t$
        \STATE Collect reward $X_t$
        \STATE Update the sum of the collected rewards within $t$ and $t-\tau+1$, namely $\hat{\mu}_{i,t,\tau}$, $T_{i,t,\tau}$ the number of pulls within $t$ and $t-\tau+1$, and $\overline{\hat{\mu}}_{i,t,\tau}=\frac{\hat{\mu}_{i,t,\tau}}{T_{i,t,\tau}}$  \label{line:updatets11}
        \STATE Update $\nu_{i,t+1} \gets \mathcal{N}(\overline{\hat{\mu}}_{i,t,\tau},\frac{1}{\gamma T_{i,t,\tau}}) $ for each $i \in \dsb{K} $
    \ENDFOR
\end{algorithmic}
\end{algorithm}
\end{minipage}
\end{figure}
\swbeta*

\begin{proof}
For ease of notation we set $\sigma_i'(T;\tau)=\sigma'_i(\tau), \overline{\mu}_{1}(\sigma_i'(T;\tau);\tau)=\overline{\mu}_{1}(\sigma'_i(\tau))$ and $\Delta_i'=\Delta_i$. For every suboptimal arm $i \in \{2,K\}$, let us define the thresholds $x_i$ and $ y_i$ s.t.~$\mu_{i}(T)< x_i < y_i < \overline{\mu}_{1}(\sigma'_i(\tau))$. Thanks to the above thresholds, we can define the following events for every $t \in {T}$:
\begin{itemize}
    \item $E^{\mu}_{i}(t)$ as the event for which ${\hat{\mu}}_{i,t,\tau} \leq x_{i}$;
    \item $E^{\theta}_{i,t}$ as the event for which $\theta_{i,t,\tau} \leq y_{i}$, where $\theta_{i,t,\tau}$ denotes a sample generated for arm $i$ from the posterior distribution at time $t$ from the sample collected in the last $\tau$ pulls, i.e., $\text{Beta}(S_{i,t,\tau} + 1, F_{i,t,\tau} + 1)$, being $S_{i,t,\tau}$ and $F_{i,t,\tau}$ the number of successes and failures from $t-\tau$ up to round $t$ for arm $i$ (note that $T_{i,t,\tau} = S_{i,t,\tau} + F_{i,t,\tau}$ and $\hat{\mu}_{i,t,\tau} = S_{i,t,\tau}/T_{i,t,\tau}$).

\end{itemize}
In the current framework we will define $p_{i,t}$ as follows:$$p_{i,t}=\Pr(\theta_{i,t,\tau}\ge y_i \mid \mathbb{F}_{t-1}).$$
Moreover, let us denote with $E^{\mu}_{i}(t)^\complement$ and $E^{\theta}_{i}(t)^\complement$ the complementary event $E^{\mu}_{i}(t)$ and $E^{\theta}_{i}(t)$, respectively. 
Let us decompose the probability term in the regret as follows:
\begin{align}
    \sum_{t=1}^{T}\Prob(I_t=i)  & =\underbrace{ \sum_{t=1}^{T} \Prob(I_t=i,E^{\mu}_{i}(t)^\complement)}_{=: P_A} + \underbrace{\sum_{t=1}^{T} \Prob(I_t=i,E^{\mu}_{i}(t),E^{\theta}_{i}(t)^\complement)}_{=: P_B} \\
    &  \quad + \underbrace{\sum_{t=1}^{T} \Prob(I_t = i, E^{\mu}_{i}(t), E^{\theta}_{i}(t))}_{=: P_C}.
\end{align}
The three terms correspond to the case of:
\begin{itemize}
    \item (i) having a poor estimation of the mean for arm $i$ (i.e., $P_A$);
    \item (ii) having a good estimation of the mean and having sampled a large value for the arm $i$ posterior sample (i.e., $P_B$);
    \item (iii) having a good estimate for the mean of the reward and having sampled a small value for the posterior sample of arm $i$ (i.e., $P_C$).
\end{itemize}
Let us analyze each term separately.

\paragraph{Term A}
We have:
\begin{align}
    P_A &= \sum_{t=1}^{T} \Prob(I_t =i, E^{\mu}_{i}(t)^\complement) \\
    & \leq \mathbb{E} \left[ \sum_{t=1}^{T}  \mathds{1} \left\{ I_t =i, E^{\mu}_{i}(t)^\complement \right\}\right]\\
    & \leq \mathbb{E} \left[ \sum_{t=1}^{T}  \mathds{1} \left\{ I_t =i, E^{\mu}_{i}(t)^\complement,T_{i,t,\tau}\leq \frac{\ln(T)}{(x_i-\mu_i(T)^2} \right\}\right]+ \nonumber\\
    +&\mathbb{E} \left[ \sum_{t=1}^{T}  \mathds{1} \left\{ I_t =i, E^{\mu}_{i}(t)^\complement,T_{i,t,\tau}\ge \frac{\ln(T)}{(x_i-\mu_i(T)))^2} \right\}\right]\\
   & \leq \frac{T\ln(T)}{\tau(x_i-\mu_i(T))^2}+\sum_{t=1}^{T}\Pr\left(E^{\mu}_{i}(t)^\complement\mid T_{i,t,\tau}\ge\frac{\ln(T)}{(x_i-\mu_i(T))^2}\right) \label{eq:chb} \\
    & \leq \frac{T\ln(T)}{\tau(x_i-\mu_i(T))^2}+\sum_{t=1}^{T}\frac{1}{T},
\end{align}
where we used the Chernoff-Hoeffding bound for the second term in Equation~\eqref{eq:chb} and Lemma~\ref{lemma:window} for the first term.

\paragraph{Term B}
Let us focus on the summands of the term $P_B$ of the regret. To this end, let $(\mathbb{F}_{t-1})_{t \in \dsb{T}}$ be the canonical filtration. We have:
\begin{align}
    \Prob( I_t = i, E^{\theta}_{i}(t)^\complement|E^{\mu}_{i}(t),\mathbb{F}_{t-1})  & \leq \Prob(\theta_{i,t,\tau}>y_{i}|\hat{\mu}_{i,t,\tau} \leq x_{i}, \mathbb{F}_{t-1}) \\
    & = \Prob \left( \text{Beta} \left( \hat{\mu}_{i,t,\tau} T_{i,t,\tau} + 1, (1 - \hat{\mu}_{i,t,\tau}) T_{i,t,\tau} + 1 \right) > y_{i} | \hat{\mu}_{i,t,\tau} \leq x_{i} \right) \label{line:line2a}\\
    & \leq \Prob \left( \text{Beta} \left( x_{i} T_{i,t,\tau} + 1, (1 - x_{i}) T_{i,t,\tau} + 1 \right) > y_{i} \right) \\
    & \leq F^{B}_{T_{i,t,\tau},y_{i}}\big(x_{i}T_{i,t,\tau}\big) \leq \exp \left( - T_{i,t,\tau} d(x_{i}, y_{i}) \right),
\end{align}
where the last inequality follows from the generalized Chernoff-Hoeffding bounds (Lemma~\ref{lemma:chernoff}) and the Beta-Binomial identity (Fact 3 of~\cite{agrawal2017near}). Equation~\eqref{line:line2a} was derived by exploiting the fact that on the event $E^{\mu}_{i}(t)$ a sample from $\text{Beta} \left( x_{i} T_{i,t,\tau} + 1, (1 - x_{i}) T_{i,t,\tau} + 1 \right) $ is likely to be as large as a sample from $Beta( \hat{\mu}_{i,t} T_{i,t,\tau}(t) + 1, (1 - \hat{\mu}_{i,t,\tau})T_{i,t,\tau} + 1 )$, reported formally in Lemma~\ref{lem:betabin}.
Therefore, for $t$ such that $T_{i,t,\tau} > L_i(T )$, where $L_i(T) \coloneqq \frac{\log{T}}{d(x_i,y_i)}$ we have:
\begin{equation}
    \Prob(I_t=i,E^{\theta}_{i}(t)^\complement|E^{\mu}_{i}(t),\mathbb{F}_{t-1})\leq\frac{1}{T}.
\end{equation}

We decompose $P_B$ in two events, when $T_{i,t,\tau} \leq L_i(T )$ and when $T_{i,t,\tau} \ge L_i(T)$ , then:
\begin{align}
    P_B & = \sum_{t=1}^{T}\Prob\big(I_t=i,E^{\mu}_{i}(t),E^{\theta}_{i}(t)^\complement \big)\leq \sum_{t=1}^{T}\Prob\big(I_t=i,E^{\theta}_{i}(t)^\complement |E^{\mu}_{i}(t)\big)\\
    & =\mathbb{E}\Big[\sum_{t=1}^{T}\Prob(I_t=i,E^{\theta}_{i}(t)^\complement|E^{\mu}_{i}(t),\mathbb{F}_{t-1}) \Big]\\
    & = \mathbb{E}\left[\mathbb{E}\Big[ \sum_{t=1}^{T} \mathds{1}(I_t=i,E^{\theta}_{i}(t)^\complement,T_{i,t,\tau}\leq L_i(T)|E^{\mu}_{i}(t),\mathbb{F}_{t-1})+\sum_{t=1}^{T} \mathds{1}(I_t=i,E^{\theta}_{i}(t)^\complement,T_{i,t,\tau}\ge L_i(T)|E^{\mu}_{i}(t),\mathbb{F}_{t-1})\Big]\right]\\ \label{eq:swcp}
    & \leq L_i(T)\frac{T}{\tau}+\E \left[ \sum_{t=1}^{T} \frac{1}{T} \right] \\
    & \leq L_i(T)\frac{T}{\tau} + 1,
\end{align}
where for the first term in Equation~\eqref{eq:swcp} we used Lemma~\ref{lemma:window}.
\paragraph{Term C}
For this term, we use Lemma~1 by~\cite{agrawal2017near}. Let us define $p_{i,t} = \Prob(\theta_{1,t,\tau} > y_i | \mathbb{F}_{t-1})$. We have:
\begin{equation}
    \Prob(I_t = i, E^{\mu}_{i}(t), E^{\theta}_{i}(t) | \mathbb{F}_{t-1}) \leq \frac{1-p_{i,t}}{p_{i,t}} \Prob(I_t = 1, E^{\mu}_{i}(t), E^{\theta}_{i}(t)|\mathbb{F}_{t-1}).
\end{equation}
Thus, we can rewrite the term $P_C$ as follows:
\begin{align}
    P_C  & = \sum_{t=1}^{T}\Prob(I_t=i,E^{\mu}_{i}(t),E^{\theta}_{i}(t)) \\
    & = \sum_{t=1}^{T} \mathbb{E}[\Prob(I_t=i,E^{\mu}_{i}(t),E^{\theta}_{i}(t)|\mathbb{F}_{t-1})] \\
    &\leq \sum_{t=1}^{T}\mathbb{E}\bigg[\mathbb{E}\bigg[\frac{1-p_{i,t}}{p_{i,t}}\mathds{1}(I_t=1,E^{\mu}_{i}(t),E^{\theta}_{i}(t))\bigg|\mathbb{F}_{t-1}\bigg]\bigg] \\
    &\leq\sum_{t=1}^{T}\mathbb{E}\bigg[\frac{1-p_{i,t}}{p_{i,t}}\mathds{1}(I_t=1,E^{\mu}_{i}(t),E^{\theta}_{i}(t))\bigg].\\
\end{align}
We rewrite the last inequality as the sum of two contributions: when the total pulls of the best arm at time $t $ $T_{1,t}>\sigma'(\tau)$ and when $T_{1,t}\leq\sigma'(\tau)$. This way, we obtain the following:
\begin{align}
    P_C\leq \underbrace{\sum_{t=1}^{T}\mathbb{E}\bigg[\frac{1-p_{i,t}}{p_{i,t}}\mathds{1}(I_t=1,E^{\mu}_{i}(t),E^{\theta}_{i}(t),T_{1,t}\leq \sigma'(\tau))\bigg]}_{A}+\nonumber\\
    +\underbrace{\sum_{t=1}^{T}\mathbb{E}\bigg[\frac{1-p_{i,t}}{p_{i,t}}\mathds{1}(I_t=1,E^{\mu}_{i}(t),E^{\theta}_{i}(t),T_{1,t}\ge \sigma'(\tau))\bigg]}_{B}.
\end{align}
We further decompose the term $A$ in other terms:
\begin{align}
    A &\leq\underbrace{\sum_{t=1}^{T}\mathbb{E}\bigg[\frac{1-p_{i,t}}{p_{i,t}}\mathds{1}\left(\overbrace{I_t=1,E^{\mu}_{i}(t),E^{\theta}_{i}(t),T_{1,t}\leq \sigma'(\tau),T_{1,t,\tau}\leq \frac{8\ln(T)}{(\overline{\mu}_1(\sigma'(\tau))-y_i)^2}}^{\mathcal{C}1}\right)\bigg]}_{(A1)} \nonumber\\
    &+\underbrace{\sum_{t=1}^{T}\mathbb{E}\bigg[\frac{1-p_{i,t}}{p_{i,t}}\mathds{1}\left(\overbrace{I_t=1,E^{\mu}_{i}(t),E^{\theta}_{i}(t),T_{1,t}\leq \sigma'(\tau),T_{1,t,\tau}\ge \frac{8\ln(T)}{(\overline{\mu}_1(\sigma'(\tau))-y_i)^2}}^{\mathcal{C}2}\right)\bigg]}_{(A2)}.
\end{align}
As $\mathbb{E}\left[XY\right] = \mathbb{E}\left[X\mathbb{E}\left[Y\mid X\right]\right]$, we can bound the term $A1$ as follows:
\begin{align}
    A1&=\sum_{t=1}^{T}\mathbb{E}\left[\mathds{1}(\mathcal{C}1)\mathbb{E}\left[\frac{1-p_{i,t}}{p_{i,t}}\mid \mathds{1}(\mathcal{C}1)\right]\right]\\
    &\leq \sum_{t=1}^{T}\mathbb{E}\left[\mathds{1}(\mathcal{C}1)\left(\frac{\delta_{TV}(P_{t\mid \mathcal{C}1},Q_{t\mid \mathcal{C}1})}{(1-\overline{\mu}_1(\sigma'(\tau)))^{\tau+1}}+\underbrace{\mathbb{E}_{\overline{\mu}_1(\sigma'(\tau))}\left[\frac{1-p_{i,t}}{p_{i,t}}\mid \mathds{1}(\mathcal{C}1)\right]}_{(*)}\right)\right].
\end{align}
Now consider an arbitrary instantiation $T_{1,t,\tau}'$ of $T_{1,t,\tau}$ (i.e., an arbitrary number of pulls of the optimal arm within the time window $\tau$) in which  $\mathcal{C}1$ holds true, we can rewrite $(*)$ as:
\begin{align}
    (*)=\mathbb{E}\left[\frac{1-p_{i,t}}{p_{i,t}}\mid \mathds{1}(C1)\right]=\mathbb{E}_{T_{1,t,\tau}'}\left[\underbrace{\mathbb{E}\left[\frac{1-p_{i,t}}{p_{i,t}}\mid \mathds{1}(C1),T_{1,t,\tau}=T_{1,t,\tau}'\right]}_{(*')}\right].
\end{align}
We can bound $(*')$ using Lemma 4 by~Agrawal et al.~\cite{agrawal2012analysis}:
\begin{align}
    &(*') = \sum_{s=0}^{T_{1,t,\tau}'}\frac{f_{T_{1,t,\tau}',\overline{\mu}_1(\sigma'(\tau))}(s)}{F_{T_{1,t,\tau}'+1,y_i}(s)}-1\nonumber\\
    &\leq \begin{cases}
    \frac{3}{\Delta_i'} & \textit{if  }  T_{1,t,\tau}'< \frac{8}{\Delta_i'}\\  
    \\
    \mathcal{O}\left(e^{-\frac{\Delta_i'^2 T_{1,t,\tau}'}{2}}+\frac{e^{-DT_{1,t,\tau}'}}{T_{1,t,\tau}'\Delta_i'^2}+\frac{1}{e^{\Delta_i'^2\frac{T_{1,t,\tau}'}{4}}-1}\right) &\textit{if  } \frac{8}{\Delta'} \leq T_{1,t,\tau}' \leq \frac{8\ln(T)}{\Delta_i'^2} \\ 
    \end{cases}.
\end{align}
We notice that the worst case scenario we can have is for $T_{i,t,\tau}'\leq\frac{8}{\Delta_i'}$ so that every possible instantiation in which condition $\mathcal{C}1$ holds true the expectation value of $\frac{1-p_{i,t}}{p_{i,t}}$ can be upper bounded by substituting in the latter inequalities the worst case scenario for $T_{i,t,\tau}'$  we obtain a term which is independent from the pulls: \begin{align}
      (*)\leq\mathcal{O}\left(\frac{1}{(\overline{\mu}_1(\sigma'(\tau))-y_i)}\right),
 \end{align}
so that the inequality for $A1$ can be rewritten as:
\begin{align}
    \mathcal{O}\left(\sum_{t=1}^T\mathds{1}(C1)(*)\right) \leq \mathcal{O}\left(\frac{T\ln(T)}{(\overline{\mu}_1(\sigma'(\tau))-y_i)^3}\right),
\end{align}
where we have exploited the fact that for Lemma~\ref{lemma:window} we have:
\begin{align}
    \sum_{t=1}^T \mathds{1}(\mathcal{C}1)\leq \frac{8T\ln(T)}{\tau(\overline{\mu}_1(\sigma'(\tau))-y_i)^2}.
\end{align}
Finally, we obtain:
\begin{align}
    A1\leq \mathcal{O}\left(\frac{\sigma'(\tau)}{ (1-\overline{\mu}_1(\sigma'(\tau)))^{\tau+1}}+\frac{T\ln(T)}{\tau (\overline{\mu}_1(\sigma'(\tau))-y_i)^3}\right),
\end{align}
Where the last inequality is a consequence of the fact that both inequalities hold:
\begin{align}
    \sum_{t=1}^{T}\mathds{1}(\mathcal{C}1)\leq\begin{cases}
        \sigma'(\tau)\\
        \\
        \frac{8T\ln(T)}{\tau(\overline{\mu}_1(\sigma'(\tau))-y_i)^2}
    \end{cases}.
\end{align}
Let us upper bound $A2$:
\begin{align}
     A2&=\sum_{t=1}^{T}\mathbb{E}\left[\mathds{1}(\mathcal{C}2)\mathbb{E}\left[\frac{1-p_{i,t}}{p_{i,t}}\mid \mathds{1}(\mathcal{C}2)\right]\right]   \\
     &\leq \sum_{t=1}^{T}\mathbb{E}\left[\mathds{1}(\mathcal{C}2)\left(\frac{\delta_{TV}(P_{t\mid \mathcal{C}2},Q_{t\mid \mathcal{C}2})}{(1-\overline{\mu}_1(\sigma'(\tau)))^{\tau+1}}+\underbrace{\mathbb{E}_{\overline{\mu}_1(\sigma'(\tau))}\left[\frac{1-p_{i,t}}{p_{i,t}}\mid \mathds{1}(\mathcal{C}2)\right]}_{(**)}\right)\right].
\end{align}
Let us consider an arbitrary instantiation $T_{1,t,\tau}'$ of $T_{1,t,\tau}$ in which $\mathcal{C}2$ holds true, i.e., an arbitrary number of pulls of the optimal arm within the time window $\tau$. We have:
\begin{align}
    (**)=\mathbb{E}\left[\frac{1-p_{i,t}}{p_{i,t}}\mid \mathds{1}(C2)\right]=\mathbb{E}_{T_{1,t,\tau}'}\left[\underbrace{\mathbb{E}\left[\frac{1-p_{i,t}}{p_{i,t}}\mid \mathds{1}(C2),T_{1,t,\tau}=T_{1,t,\tau}'\right]}_{(**')}\right],
\end{align}
where we bound the term $(**')$ using Lemma~4 by~Agrawal et al.~\cite{agrawal2012analysis}:
\begin{align}
   &(**') = \sum_{s=0}^{T_{1,t,\tau}'}\frac{f_{T_{1,t,\tau}',\overline{\mu}_1(\sigma'(\tau))}(s)}{F_{T_{1,t,\tau}'+1,y_i}(s)}-1\nonumber\\ &\leq \mathcal{O}\left(e^{-\frac{\Delta_i'^2 T_{1,t,\tau}'}{2}}+\frac{e^{-DT_{1,t,\tau}'}}{T_{1,t,\tau}'\Delta_i'^2}+\frac{1}{e^{\Delta_i'^2\frac{T_{1,t,\tau}'}{4}}-1}\right) \textit{ for } T_{1,t,\tau}'\ge \frac{8\ln(T)}{\Delta_i'^2}.
\end{align}
We see that the worst case scenario when $\mathcal{C}2$ holds true is when $ T_{i,t,\tau}'= \frac{8\ln(T)}{\Delta_i'^2}$, so considering the worst case scenario for the case $\mathcal{C}2$ holds true we can bound the expected value for $\frac{1-p_{i,t}}{p_{i,t}}$ for every possible realization of $\mathcal{C}2$ independently from $T_{1,t,\tau}'$ as:
\begin{align}
    (**)\leq \mathcal{O}\left( \frac{1}{T-1}\right)\leq  \mathcal{O}\left( \frac{1}{T}\right),
\end{align}
so that:
\begin{align}
  A2\leq \mathcal{O}\left(\frac{\sigma'(\tau)}{ (1-\overline{\mu}_1(\sigma'(\tau)))^{\tau+1}}\right),
\end{align}
where the latter inequality is a consequence of the fact that:
\begin{align}
    \sum_{t=1}^{T}\mathds{1}(\mathcal{C}2)\leq \sigma'(\tau).
\end{align}
Let us bound term $B$. We decompose this term in two contributions:
\begin{align}
    B=\sum_{t=1}^{T}\mathbb{E}\bigg[\frac{1-p_{i,t}}{p_{i,t}}\mathds{1}(I_t=1,E^{\mu}_{i}(t),E^{\theta}_{i}(t),T_{1,t}\ge \sigma'(\tau))\bigg],
   \end{align}
so that, similarly to what we have done earlier, we have:
\begin{align}
    B = \underbrace{\sum_{t=1}^{T}\mathbb{E}\bigg[\frac{1-p_{i,t}}{p_{i,t}}\mathds{1}\left(\overbrace{I_t=1,E^{\mu}_{i}(t),E^{\theta}_{i}(t),T_{1,t}\ge \sigma'(\tau),T_{1,t,\tau}\leq \frac{8\ln(T)}{(\overline{\mu}_1(\sigma'(\tau))-y_i)^2}}^{\mathcal{C}1'}\right)\bigg]}_{B1}+ \nonumber\\
    +\underbrace{\sum_{t=1}^{T}\mathbb{E}\bigg[\frac{1-p_{i,t}}{p_{i,t}}\mathds{1}\left(\overbrace{I_t=1,E^{\mu}_{i}(t),E^{\theta}_{i}(t),T_{1,t}\ge \sigma'(\tau),T_{1,t,\tau}\ge \frac{8\ln(T)}{(\overline{\mu}_1(\sigma'(\tau))-y_i)^2}}^{\mathcal{C}2'}\right)\bigg]}_{B_2}.
\end{align}
Let us deal with $B1$ first. We have:
\begin{align}
    B1 = \sum_{t=1}^{T}\mathbb{E}\left[\mathds{1}(\mathcal{C}1')\underbrace{\mathbb{E}\left[\frac{1-p_{i,t}}{p_{i,t}}\mid \mathds{1}(\mathcal{C}1')\right]}_{(*)}\right].
\end{align}
Let us analyse $(*)$ first.
\begin{align}
    (*)\leq \mathbb{E}_{T_{1,t,\tau}'}\left[\mathbb{E}\underbrace{\left[\frac{1-p_{i,t}}{p_{i,t}}\mid \mathds{1}(\mathcal{C}1'), T_{1,t,\tau}=T_{1,t,\tau}'\right]}_{(**)}\right]
\end{align}

Lemma~\ref{lemma:techlemma} applied to $(**)$, states that a bound for a $\text{Bin}(T_{1,t,\tau}',\mu_1(\sigma'(\tau)))$, i.e., binomial process with parameters $T_{1,t,\tau}'$ and $\mu_1(\sigma'(\tau))$ holds also for $(**)$, since such a Poisson-binomial has a mean equal or larger than $\overline{\mu}_1(\sigma'(\tau))$).
It follows, applying Lemma 4 by~\cite{agrawal2012analysis} to $(**)$, we have that:
$$(**) \leq \mathcal{O}\left(\frac{1}{(\overline{\mu}_1(\sigma'(\tau))-y_i)}\right).$$
Therefore we have by Lemma~\ref{lemma:window}:
\begin{align}
    \sum_{t=1}^{T}\mathds{1}(\mathcal{C}1')\leq \mathcal{O}\left(\frac{T\ln(T)}{\tau(\overline{\mu}_1(\sigma'(\tau))-y_i)^2}\right).
\end{align}

Finally, we obtain that:
\begin{align}
    B1 \leq \mathcal{O}\left(\frac{T\ln(T)}{\tau(\overline{\mu}_1(\sigma'(\tau))-y_i)^3}\right),
\end{align}
where the above inequality follows from Lemma~\ref{lemma:window}.

Let us analyse $B2$:
\begin{align}
    B2=\sum_{t=1}^{T}\mathbb{E}\left[\mathds{1}(\mathcal{C}2')\underbrace{\mathbb{E}\left[\frac{1-p_{i,t}}{p_{i,t}}\mid \mathds{1}(\mathcal{C}2')\right]}_{(*')}\right].
\end{align}
Similarly to what has been done for term B1, applying Lemma~\ref{lemma:techlemma} to $(*')$, we have that that term can be bounded by the same bound we would have for a process governed by a Binomial distribution $\text{Bin}(\cdot,\overline{\mu}_1(\sigma'(\tau)))$. Thus, applying Lemma 4 by~\cite{agrawal2012analysis} to such a distribution :
$$(*') \leq \mathcal{O}\left(\frac{1}{T}\right),$$
and, finally:
\begin{align}
    B2\leq \mathcal{O}(1).
\end{align}

Choosing $x_i=\mu_i(T)+\frac{\Delta_i}{3}$ and $y_i=\overline{\mu}_1(\sigma'(\tau))-\frac{\Delta_i}{3}$ and summing all the term concludes the proof.
\end{proof}

\gtssw*

\begin{proof}
For ease of notation we set $\sigma_i'(T;\tau)=\sigma'_i(\tau), \overline{\mu}_{1}(\sigma_i'(T;\tau);\tau)=\overline{\mu}_{1}(\sigma'_i(\tau))$ and $\Delta_i'=\Delta_i$. For every suboptimal arm $i \in \{2,K\}$, let us define the thresholds $x_i$ and $ y_i$ s.t.~$\mu_{i}(T)< x_i < y_i < \overline{\mu}_{1}(\sigma'_i(\tau))$. Thanks to the above thresholds, we can define the following events for every $t \in {T}$:
\begin{itemize}
    \item $E^{\mu}_{i}(t)$ as the event for which $\overline{\hat{\mu}}_{i,t,\tau} \leq x_{i}$;
    \item $E^{\theta}_{i,t}$ as the event for which $\theta_{i,t,\tau} \leq y_{i}$, where $\theta_{i,t,\tau}$ denotes a sample generated for arm $i$ from the posterior distribution at time $t$ , i.e., $\mathcal{N}(\overline{\hat{\mu}}_{i,t},\frac{1}{\gamma T_{i_t,t,\tau}})$, being $T_{i_t,t}$  of trials at time $t$ in the temporal window $\tau$ for arm $i_t$.
\end{itemize}
In such a framework $p_{i,t}$ is defined as $p_{i,t}=\Pr(\theta_{i,t,\tau}\ge y_i \mid \mathbb{F}_{t-1})$
Moreover, let us denote with $E^{\mu}_{i}(t)^\complement$ and $E^{\theta}_{i}(t)^\complement$ the complementary event $E^{\mu}_{i}(t)$ and $E^{\theta}_{i}(t)$, respectively.
Let us focus on decomposing the probability term in the regret as follows:
\begin{align}
    \sum_{t=1}^T\Prob(I_t=i)  & =\underbrace{ \sum_{t=1}^T\Prob(I_t=i,E^{\mu}_{i}(t)^\complement)}_{=: P_A} + \underbrace{\sum_{t=1}^T\Prob(I_t=i,E^{\mu}_{i}(t),E^{\theta}_{i}(t)^\complement)}_{=: P_B} \\
    &  \quad + \underbrace{\sum_{t=1}^T\Prob(I_t = i, E^{\mu}_{i}(t), E^{\theta}_{i}(t))}_{=: P_C}.
\end{align}
Let us analyze each term separately.

\paragraph{Term A}
We have:
\begin{align}
    P_A &= \sum_{t=1}^{T} \Prob(I_t =i, E^{\mu}_{i}(t)^\complement) \\
    & \leq \mathbb{E} \left[ \sum_{t=1}^T  \mathds{1} \left\{ I_t =i, E^{\mu}_{i}(t)^\complement \right\}\right]\\
    & \leq \mathbb{E} \left[ \sum_{t=1}^T  \mathds{1} \left\{ I_t =i, E^{\mu}_{i}(t)^\complement,T_{i,t,\tau}\leq \frac{\ln(T\Delta_i^2+e)}{\gamma(x_i-\mu_i(T))^2} \right\}\right]+ \nonumber\\ &+\mathbb{E} \left[ \sum_{t=1}^T \mathds{1} \left\{ I_t =i, E^{\mu}_{i}(t)^\complement,T_{i,t,\tau}\ge \frac{\ln(T\Delta_i^2+e)}{\gamma(x_i-\mu_i(T))^2} \right\}\right]\\
   & \leq \frac{T\ln(T\Delta_i^2+e)}{\gamma\tau(x_i-\mu_i(T))^2}+\sum_{t=1}^T\Pr\left(E^{\mu}_{i}(t)^\complement\mid T_{i,t,\tau}\ge\frac{\ln(T\Delta_i^2+e)}{\gamma(x_i-\mu_i(T))^2}\right) \\
    & \leq \frac{T\ln(T\Delta_i^2+e)}{\gamma\tau(x_i-\mu_i(T))^2}+\sum_{t=1}^T\frac{1}{T\Delta_i^2},
\end{align}
Where we used Lemma~\ref{lemma:window} and Lemma~\ref{lemma:Subg} as we did in the proof of Theorem~\ref{thm:gts}.

\paragraph{Term B}
Defining $L_i(T)=\frac{288\log(T\Delta_i^2+e^{6})}{\gamma \Delta_i^2}$, we decompose each summand into two parts:
\begin{align}
    P_B & = \sum_{t=1}^T\Prob\big(I_t=i,E^{\mu}_{i}(t),E^{\theta}_{i}(t)^\complement \big)\\
    &=\sum_{t=1}^T\Prob\big(I_t=i,T_{i,t,\tau}\leq L_i(T), E^{\mu}_{i}(t),E^{\theta}_{i}(t)^\complement \big)+\Prob\big(I_t=i,T_{i,t,\tau} >L_i(T), E^{\mu}_{i}(t),E^{\theta}_{i}(t)^\complement \big).
\end{align}
The first term is bounded by $L_i(T)\frac{T}{\tau}$ using Lemma~\ref{lemma:window}. Instead, regarding the second term:
\begin{align}
    & \sum_{t=1}^T \Prob\left(i(t)=i, T_{i,t,\tau}>L_i(\tau), E_i^\theta(t)^\complement, E_i^\mu(t)\right)\\
    & \leq \mathbb{E}\left[\sum_{t=1}^T \Prob\left(i(t)=i, {E_i^\theta(t)}^\complement \mid T_{i,t,\tau}>L_i(T), E_i^\mu(t), \mathbb{F}_{t-1}\right)\right] \\
    & \leq \mathbb{E}\left[\sum_{t=1}^T \Prob\left(\theta_{i,t,\tau}>y_i \mid T_{i,t,\tau}>L_i(T), \overline{\hat{\mu}}_{i,t,\tau} \leq x_i, \mathbb{F}_{t-1}\right)\right].
\end{align}
In this setting, $\theta_{i,t,\tau}$ is a Gaussian random variable distributed as $\mathcal{N}\left(\overline{\hat{\mu}}_{i,t,\tau}, \frac{1}{\gamma T_{i,t,\tau}}\right)$. We recall that an $\mathcal{N}\left(m, \sigma^2\right)$ distributed r.v. ~(i.e., a Gaussian random variable with mean $m$ and variance $\sigma^2$ ) is stochastically dominated by $\mathcal{N}\left(m^{\prime}, \sigma^2\right)$ distributed r.v.~if $m^{\prime} \geq m$. Therefore, given $\overline{\hat{\mu}}_{i,t,\tau} \leq x_i$, the distribution of $\theta_{i,t,\tau}$ is stochastically dominated by $\mathcal{N}\left(x_i, \frac{1}{\gamma T_{i,t,\tau}}\right)$. Formally:
\begin{equation} \label{eq:domi}
\Prob\left(\theta_{i,t,\tau}>y_i \mid T_{i,t,\tau}>L_i(T), \overline{\hat{\mu}}_{i,t,\tau} \leq x_i, \mathbb{F}_{t-1}\right) \leq \Prob\left(\left.\mathcal{N}\left(x_i, \frac{1}{\gamma T_{i,t,\tau}}\right)>y_i \right\rvert\, \mathbb{F}_{t-1}, T_{i,t,\tau}>L_i(T)\right) .
\end{equation}

Using Lemma \ref{lemma:Abramowitz2} we have:
\begin{align} \Prob\left(\mathcal{N}\left(x_i, \frac{1}{\gamma T_{i,t,\tau}}\right)>y_i\right) & \leq \frac{1}{2} e^{-\frac{\left(\gamma T_{i,t,\tau}\right)\left(y_i-x_i\right)^2}{2}} \\ & \leq \frac{1}{2} e^{-\frac{\left(\gamma L_i(T)\right)\left(y_i-x_i\right)^2}{2}}\end{align}
which is smaller than $\frac{1}{T \Delta_i^2}$ because $L_i(T) \geq \frac{2 \ln \left(T \Delta_i^2\right)}{\gamma \left(y_i-x_i\right)^2}$. Substituting into Equation~\eqref{eq:domi}, we get:
\begin{equation}
   \Prob\left(\theta_{i,t,\tau}>y_i \mid T_{i,t,\tau}>L_i(T), \overline{\hat{\mu}}_{i,t,\tau} \leq x_i, \mathbb{F}_{t-1}\right)  \leq \frac{1}{T\Delta_i^2}.
\end{equation}
Summing over $t$ follows that $P_B \leq O \left(\frac{T}{\tau}L_i(T)+\frac{1}{\Delta_i^2}\right)$.

\paragraph{Term C}
For this term, we use Lemma~1 by~\cite{agrawal2017near}. Let us define $p_{i,t} := \Prob(\theta_{1,t,\tau} > y_i | \mathbb{F}_{t-1})$. We have:
\begin{equation}
    \Prob(I_t = i, E^{\mu}_{i}(t), E^{\theta}_{i}(t) | \mathbb{F}_{t-1}) \leq \frac{1-p_{i,t}}{p_{i,t}} \Prob(I_t = 1, E^{\mu}_{i}(t), E^{\theta}_{i}(t)|\mathbb{F}_{t-1}).
\end{equation}
Thus, we can rewrite the term $P_C$ as follows:
\begin{align}
    P_C  & = \sum_{t=1}^T\Prob(I_t=i,E^{\mu}_{i}(t),E^{\theta}_{i}(t)) \\
    & =\sum_{t=1}^T \mathbb{E}[\Prob(I_t=i,E^{\mu}_{i}(t),E^{\theta}_{i}(t)|\mathbb{F}_{t-1})] \\
    &\leq \sum_{t=1}^T\mathbb{E}\bigg[\mathbb{E}\bigg[\frac{1-p_{i,t}}{p_{i,t}}\mathds{1}(I_t=1,E^{\mu}_{i}(t),E^{\theta}_{i}(t))\bigg|\mathbb{F}_{t-1}\bigg]\bigg] \\
    &\leq\sum_{t=1}^T\mathbb{E}\bigg[\frac{1-p_{i,t}}{p_{i,t}}\mathds{1}(I_t=1,E^{\mu}_{i}(t),E^{\theta}_{i}(t))\bigg].\label{eq:lastin}
\end{align}
We decompose Equation~\eqref{eq:lastin} into two contributions:
\begin{align}
   P_C \leq \underbrace{\sum_{t=1}^T\mathbb{E}\bigg[\frac{1-p_{i,t}}{p_{i,t}}\mathds{1}(I_t=1,E^{\mu}_{i}(t),E^{\theta}_{i}(t), T_{1,t}\leq \sigma'(\tau))\bigg]}_{B1}+\nonumber\\+\underbrace{\sum_{t=1}^T\mathbb{E}\bigg[\frac{1-p_{i,t}}{p_{i,t}}\mathds{1}(I_t=1,E^{\mu}_{i}(t),E^{\theta}_{i}(t), T_{1,t}\geq \sigma'(\tau))\bigg]}_{A1}.
\end{align}
Analyzing term $A1$:
\begin{align}
    A1 \leq \underbrace{\sum_{t=1}^T\mathbb{E}\bigg[\frac{1-p_{i,t}}{p_{i,t}}\mathds{1}\left(\overbrace{I_t=1,E^{\mu}_{i}(t),E^{\theta}_{i}(t),T_{1,t,\tau}\leq L_i(T), T_{1,t}\geq \sigma'(\tau)}^{\mathcal{C}1}\right)\bigg]}_{A}+\nonumber\\+\underbrace{\sum_{t=1}^T\mathbb{E}\bigg[\frac{1-p_{i,t}}{p_{i,t}}\mathds{1}\left(\overbrace{I_t=1,E^{\mu}_{i}(t),E^{\theta}_{i}(t),T_{1,t,\tau}\ge L_i(T), T_{1,t}\geq \sigma'(\tau)}^{\mathcal{C}2}\right)\bigg]}_{B} \label{eq:c1def}
\end{align}
Let us tackle the term $A$ by exploiting the fact that $\mathbb{E}[XY]=\mathbb{E}[X\mathbb{E}[Y\mid X]]$. This way, we can rewrite it as:
\begin{align}\label{eq:rippop}
    A=\sum_{t=1}^T\mathbb{E}\left[\mathds{1}(\mathcal{C}1)\underbrace{\mathbb{E}\left[\frac{1-p_{i,t}}{p_{i,t}}\mid \mathds{1}(\mathcal{C}1)\right]}_{(*)}\right].
\end{align}

%i.e., the number of times we have already played the optimal arm ($T_{1,t}\ge \sigma'(\tau)$) is such that the rewards produced are sampled with a probability of success bigger than $\overline{\mu}_1(\sigma'(\tau))$,
In the following, we show that whenever condition $\mathcal{C}1$ holds $(*)$ is bounded by a constant. Let $\Theta_j$ denote a $\mathcal{N}\left(\overline{\hat{\mu}}_{1,j}, \frac{1}{\gamma j}\right)$ distributed Gaussian random variable, where $\overline{\hat{\mu}}_{1,j}$ is the sample mean of the optimal arm's rewards played $j$ times within a time window $\tau$. Let $G_j$ be a geometric random variable denoting the number of consecutive independent trials up to $j$ included where a sample of $\Theta_j$ is greater than $y_i$. We will show that for any realization of the number of pulls within a time window $\tau$ such that condition $\mathcal{C}1$ holds, the expected value of $G_j$ is bounded by a constant for all $j$.

Consider an arbitrary realization of $T_{1,t,\tau} = j$ that satisfies condition $\mathcal{C}1$. Observe that $p_{i,t}=\operatorname{Pr}\left(\Theta_j>y_i \mid \mathbb{F}_{\tau_j}\right)$ and:
\begin{align}
    \mathbb{E}\left[\frac{1}{p_{i, t}}\mid \mathds{1}(\mathcal{C}1)\right]= \mathbb{E}_{j}\left[\mathbb{E}\left[\frac{1}{p_{i, t}}\mid \mathds{1}(\mathcal{C}1), T_{1,t,\tau}=j\right]\right]=\mathbb{E}_{j_{\mid \mathcal{C}1}}\left[\mathbb{E}\left[\mathbb{E}\left[G_j \mid \mathbb{F}_{\tau_j}\right]\right]\right]=\mathbb{E}_{j_{\mid \mathcal{C}1}}\left[\mathbb{E}\left[G_j\right]\right]. \label{eq:expgj}
\end{align}
Notice that the term $\mathbb{E}\left[G_j\right]$ in Equation~\eqref{eq:expgj} is the same as the one we had in Equation~\eqref{eq:rif} to derive bounds for the $\gamma$-\texttt{GTS} algortihtm. Relying on the same mathematical steps we bound it as follows:
$$\mathbb{E}\left[G_j\right] \leq e^{12}+5.$$
This shows a constant bound independent from $j$ of $\mathbb{E}\left[\frac{1}{p_{i, t}}-1\right]$ for any $j$ such that condition $\mathcal{C}1$ holds. Then, using Lemma~\ref{lemma:window}, $A$ can be rewritten as:
\begin{align}
    A&\leq (e^{12}+5)\mathbb{E}\left[\sum_{t=1}^T\mathds{1}(\mathcal{C}1)\right]\\
    &\leq (e^{12}+5)\frac{288T\ln(T\Delta_i^2+e^6)}{\gamma\tau\Delta_i^2}.
\end{align}
Let us tackle $B$ by exploiting the fact that $\mathbb{E}[XY]=\mathbb{E}[X\mathbb{E}[Y\mid X]]$:
\begin{align}\label{eq:ripopp2}
    B=\sum_{t=1}^T\mathbb{E}\left[\mathds{1}(\mathcal{C}2)\underbrace{\mathbb{E}\left[\frac{1-p_{i,t}}{p_{i,t}}\mid \mathds{1}(\mathcal{C}2)\right]}_{(**)}\right].
\end{align}
We derive a  bound for $(**)$ for large $j$ as imposed by condition $\mathcal{C}2$. Consider then an arbitrary case in which $T_{i,t,\tau} = j \geq L_i(T)$ (as dictated by $\mathcal{C}2$), we have:
\begin{align}
    \mathbb{E}\left[\frac{1}{p_{i, t}}\mid \mathds{1}(\mathcal{C}2)\right]= \mathbb{E}_{j}\left[\mathbb{E}\left[\frac{1}{p_{i, t}}\mid \mathds{1}(\mathcal{C}2), T_{1,t,\tau}=j\right]\right]=\mathbb{E}_{j_{\mid \mathcal{C}2}}\left[\mathbb{E}\left[\mathbb{E}\left[G_j \mid \mathbb{F}_{\tau_j}\right]\right]\right]=\mathbb{E}_{j_{\mid \mathcal{C}2}}\left[\mathbb{E}\left[G_j\right]\right].
\end{align}

Notice that the term $\mathbb{E}\left[G_j\right]$ in the last equation is the same that bounded in Theorem~\ref{thm:gts} for the regret of $\gamma$-\texttt{GTS}. Therefore, using the same proof line it is bounded by $\mathbb{E}\left[G_j\right] \leq \frac{1}{T\Delta_i^2}$.

For term $B1$, we made the same passages that we did for Equations~\eqref{eq:rippop} and~\eqref{eq:ripopp2}, adding the $\delta_{TV}(\cdot,\cdot)$ term, yielding to:
\begin{equation}
    B1 \leq O \left( \frac{\sigma'(\tau)}{(1 - \bar{\mu}(\sigma'(\tau)))^{\tau+1}}) + (e^{12}+5)\frac{288T\ln(T\Delta_i^2+e^6)}{\gamma\tau\Delta_i^2} + \frac{1}{\Delta_i^2} \right),
\end{equation}
and summing up the terms concludes the proof.
\end{proof}

\clearpage
\section{Auxiliary Lemmas}
In this section, we report some results that already exist in the bandit literature and have been used to demonstrate our results.

\begin{restatable}[Generalized Chernoff-Hoeffding bound from~\cite{agrawal2017near}]{lemma}{chernoff}\label{lemma:chernoff}
Let $X_1, \ldots , X_n$ be independent Bernoulli random variables with $\mathbb{E}[X_i
] = p_i$, consider the random variable $X = \frac{1}{n}\sum_{i=1}^nX_i$, with $\mu = \mathbb{E}[X]$.
For any $0 < \lambda < 1 - \mu$ we have:
\[
\Prob(X\ge\mu+\lambda)\leq \exp{\big(-nd(\mu+\lambda,\mu)\big)},
\]
and for any $0 < \lambda < \mu$
\[
\Prob(X\leq\mu-\lambda)\leq \exp{\big(-nd(\mu-\lambda,\mu)\big)},
\]
where $d(a, b) \coloneqq a \ln{\frac{a}{b}} + (1-a) \ln{\frac{1-a}{1-b}}$.
\end{restatable}

\begin{restatable}[Change of Measure Argument from~\cite{lattimore2020bandit}]{lemma}{distance}\label{lemma:changeMeasure}
Let $(\Omega, \mathcal{F})$ be a measurable space, and $P, Q: \mathcal{F}\rightarrow [0,1]$. Let $a < b$ and $X \rightarrow [a, b]$ be a $\mathcal{F}$-measurable random variable, we have:
\begin{equation}
    \left| \int_{\Omega} X(\omega) \,dP(\omega) \ - \int_{\Omega} X(\omega) \,dQ(\omega) \right| \leq (b-a)\delta_{TV}(P,Q).
\end{equation}
\end{restatable}
\begin{restatable}[\cite{lattimore2020bandit}, proposition 2.8]{lemma}{mean}\label{lemma:change}
    For a nonnegative random variable $X$, the expected value $\mathbb{E}[X]$ can be computed as:
\[
\mathbb{E}[X] = \int_{0}^{\infty} Pr(X \ge y)dy.
\]
\end{restatable}

\begin{restatable}[\cite{roos2001binomialapproximation}, Theorem 2]{lemma}{deltadistancepb} \label{lemma:delta}
Let us define $\underline{\mu}_n \coloneqq (\mu_1, \ldots, \mu_{n})$, $s \in (0, \ldots, n)$ and $\mu \in (0,1)$. We have that the total variation distance between two variables $PB(\underline{\mu}_{n})$ and $B_s(n, \mu)$ is:
\begin{equation}
     \delta_{TV}(PB(\underline{\mu}_{n}), B_s(n,\mu)) \leq
     \begin{cases}
        C_1(s) \theta(\mu,\underline{\mu}_n)^{\frac{s+1}{2}} \frac{\left(1-\frac{s}{s+1}\sqrt{\theta(\mu,\underline{\mu}_n)}\right)}{(1-\sqrt{\theta (\mu,\underline{\mu}_n)})^2} &\text{if } \theta(\mu,\underline{\mu}_n)< 1\\
        C_2(s) \eta(\mu,\underline{\mu}_n)^{\frac{s+1}{2}}(1+\sqrt{2\eta(\mu,\underline{\mu}_n)})\exp(2\eta(\mu,\underline{\mu}_n)) &\text{otherwise }
    \end{cases},
\end{equation}
where $\theta(\mu, \underline{\mu}_n) \coloneqq \frac{\eta(\mu, \underline{\mu}_n)}{2 n \mu (1 - \mu)}$, $\eta(\mu, \underline{\mu}_n) \coloneqq 2 \gamma_{2}(\mu, \underline{\mu}_n) + \gamma_{1}(\mu, \underline{\mu}_n)^2$, $\gamma_{k}(\mu, \underline{\mu}_n) \coloneqq \sum_{n'=1}^{n} (\mu - \mu_{n'})^k$, $C_{1}(s) \coloneqq \frac{\sqrt{e}(s+1)^{\frac{1}{4}}}{2}$, $C_2(s) \coloneqq \frac{(2\pi)^{\frac{1}{4}} \exp{(\frac{1}{24(s+1)}})2^{\frac{s-1}{2}}}{\sqrt{s!}(s+1)^{\frac{1}{4}}}$.
\end{restatable}

%{\color{green} al limite scriviamo un corollario per $s=0$}
%where we do highlight that $B_{s=0}(n,p)$ it's just the binomial distribution with $n$ trials and probability $p$ of success of each trial $Bin(n,p)$.

\begin{restatable}[\cite{ehm1997binomial}, Theorem 1, Lemma 2] {lemma}{deltadistance} \label{lemma:deltadistance}
    Using the quantities defined in the Lemma \ref{lemma:delta},
    \begin{equation}
        \frac{\theta(\overline{\mu},\underline{\mu}_n)}{124}\min\{1,n\overline{\mu}(1-\overline{\mu})\}\leq\delta_{TV}(PB(\underline{\mu}_n),Bin(n,\overline{\mu})))\leq \frac{1-\overline{\mu}^{n+1}-(1-\overline{\mu})^{n+1}}{(n+1)\overline{\mu}(1-\overline{\mu})} \gamma_2(\overline{\mu},\underline{\mu}_n)
    \end{equation}
where $\overline{\mu}$ is the mean of the components of the means' vector $\underline{\mu}_n$, i.e. $\overline{\mu}=\frac{\sum_{n'=1}^n \mu_{n'}}{n}$
\end{restatable}

\begin{restatable}[Beta-Binomial identity]{lemma}{betabin} \label{lem:betabin}
    For all positive integers $\alpha, \beta \in \mathbb{N}$, the following equality holds:
    \begin{equation}
        F_{\alpha, \beta}^{beta}(y) = 1 - F_{\alpha + \beta - 1, y}^B(\alpha - 1),
    \end{equation}
    where $F_{\alpha, \beta}^{beta}(y)$ is the cumulative distribution function of a beta with parameters $\alpha$ and $\beta$, and $F_{\alpha + \beta - 1, y}^B(\alpha - 1)$ is the cumulative distribution function of a binomial variable with $\alpha + \beta - 1$ trials having each probability $y$.
\end{restatable}

\begin{restatable}
    [\cite{boland2002stochastic}, Theorem 1 (iii)] {lemma}{stochastic} \label{lemma:stochastic}
    Let $Y \sim Bin(n,\lambda)$ and $X=\sum X_i$ where the $X_i \sim Bin(n_i,\lambda_i)$ are independent random variables for $i=1,\ldots,k$ then:
    \begin{align}
        & X \ge_{st}Y \textit{if and only if } \lambda\leq\overline{\lambda}_g, \\
        & X \leq_{st}Y \textit{if and only if } \lambda\ge\overline{\lambda}_{cg}, 
    \end{align}
    where $X\ge_{st}Y$ means that $X$ is greater than $Y$ in the stochastic order, i.e. $Pr(X\ge m)\ge Pr(Y\ge m) \text{ }\forall m $, and:
    \begin{align}
        & \overline{\lambda}_g =\left(\prod_{i=1}^k\lambda_i^{n_i}\right)^{\frac{1}{n}}, \\
        & \overline{\lambda}_{cg} =1-\left(\prod_{i=1}^k(1-\lambda_i)^{n_i}\right)^{\frac{1}{n}}.
    \end{align}
\end{restatable}

\begin{restatable}[\cite{abramowitz1968handbook} Formula $7.1.13$]{lemma}{Abramowitz}\label{lemma:Abramowitz}
Let $Z$ be a Gaussian random variable with mean $\mu$ and standard deviation $\sigma$, then:
\begin{equation}
    \Prob(Z>\mu+x\sigma)\ge \frac{1}{\sqrt{2\pi}}\frac{x}{x^2+1}e^{-\frac{x^2}{2}}
\end{equation}
\end{restatable}

\begin{restatable}[\cite{abramowitz1968handbook}]{lemma}{Abramowitz2}\label{lemma:Abramowitz2}
Let $Z$ be a Gaussian r.v.~with mean $m$ and standard deviation $\sigma$, then:
    \begin{equation}
        \frac{1}{4 \sqrt{\pi}} e^{-7 z^2 / 2}<\Prob(|Z-m|>z \sigma) \leq \frac{1}{2} e^{-z^2 / 2}.
    \end{equation}
\end{restatable}

\begin{restatable}[\cite{rigollet2023high} Corollary $1.7$]{lemma}{Subg}\label{lemma:Subg}
Let $X_1,\ldots, X_n$ be $n$ independent random variables such that $X_i\sim $ \textsc{Subg}($\sigma^2$), then for any $a \in \mathbb{R}^n$, we have
\begin{equation}
\Prob\left[\sum_{i=1}^n a_i X_i>t\right] \leq \exp \left(-\frac{t^2}{2 \sigma^2|a|_2^2}\right),    
\end{equation}

and
\begin{equation}
    \Prob\left[\sum_{i=1}^n a_i X_i<-t\right] \leq \exp \left(-\frac{t^2}{2 \sigma^2|a|_2^2}\right)
\end{equation}

Of special interest is the case where $a_i=1 / n$ for all $i$ we get that the average $\bar{X}=\frac{1}{n} \sum_{i=1}^n X_i$, satisfies
$$
\Prob(\bar{X}>t) \leq e^{-\frac{n t^2}{2 \sigma^2}} \quad \text { and } \quad \mathbb{P}(\bar{X}<-t) \leq e^{-\frac{n t^2}{2 \sigma^2}}
$$
\end{restatable}
\begin{restatable}[\cite{hoeffding1956trials},\cite{tang2023pb}, Theorem 2.1 (2)]{lemma}{hoeffpomp}\label{lemma:hoeffpomp}
Let $X \sim \operatorname{PB}\left(p_1, \ldots, p_n\right)$, and $\bar{X} \sim \operatorname{Bin}(n, \bar{p})$, for any convex function $g:[n] \rightarrow \mathbb{R}$ in the sense that $g(k+2)-2 g(k+1)+g(k)>0$, $0 \leq k \leq n-2$, we have
\begin{equation}
    \mathbb{E} g(X) \leq \mathbb{E} g(\bar{X}),
\end{equation}

where the equality holds if and only if $p_1=\cdots=p_n$ of the poisson-binomial distribution are all equal to $\bar{p}$ of the binomial.
\end{restatable}
\begin{restatable}[Bretagnolle-Hubner inequality]{fact}{bh} \label{fact:BH}
The Bretagnolle-Huber inequality states:
\begin{equation}
 \delta_{\mathrm{TV}}(P, Q) \leq \sqrt{1-\exp \left(-D_{\mathrm{KL}}(P \| Q)\right)} \leq 1-\frac{1}{2} \exp \left(-D_{\mathrm{KL}}(P \| Q)\right)   
\end{equation}
\end{restatable}
\begin{restatable}[\cite{Johnson_2006} Definition 1.2, \cite{HOGGAR1974concavity} ] {lemma}{con}\label{lemma:con}
A random variable V taking values in $\mathbb{Z}_+$ is discrete log-concave if its probability
mass function $p_V (i) = P(V = i)$ forms a log-concave sequence. That is, $V$ is log-concave
if for all $i \ge 1$:
\begin{align}
    p_V(i)^2 \ge p_V(i-1) p_V(i+1)
\end{align}
Any Bernoulli random variable (that is, only taking values in $\{0, 1\}$) is discrete log-concave.
Further, any binomial distribution is discrete log-concave. In fact any random variable $S = \sum_{i=1}^n X_i$, where $X_i$ are independent (not necessarily identical) Bernoulli variables, is discrete log-concave. Notice then that by definition $\frac{1}{p_V(i)}$ is discret log-convex
\end{restatable}
\begin{restatable}[\cite{Hill1999AdvancesIS}, Theorem 2 p.152, Remark 13 p.153, Remark 1 p.150] {lemma}{logcon} \label{lemma:logcon}
 Let $1 \leq \alpha<r \leq \infty$ and let $q: \mathbb{Z} \rightarrow[0, \infty]$ be $r$-concave (Definition $1$ p.150 \cite{Hill1999AdvancesIS}, furthermore we highlight that for Remark 1 p.150 \cite{Hill1999AdvancesIS} to be $\infty$-concave is equivalent to be discrete log-concave). Then $\mathcal{J}^\alpha {q}$ is $(r-\alpha)$-concave, we assume $r-\alpha=\infty$ when $r=\infty$ and $r>\alpha$. Where the $\alpha$-fractional (tail) sum of a function $q: \mathbb{Z} \rightarrow [0,\infty]$ is defined for every $\alpha> 0$ by the formula:
 \begin{align}
     \mathcal{J}^\alpha {q}(n)=\sum_{k=0}^{\infty} \binom{\alpha+k-1}{k} q(n+k),
 \end{align}
 so that for a binomial pdf $p_{\textit{bin}}$, being $p_{\textit{bin}}$ discrete log-concave (see \ref{lemma:con}), follows that $\mathcal{J}^\alpha p_{\textit{bin}}$ is $\infty$-concave on $\mathbb{Z}$ for $\alpha \ge 1$.
\end{restatable}

\begin{restatable}[\cite{combes2014unimodal}, Lemma D.1]{lemma}{combprot}\label{lemma:window}
     Let $A \subset \mathbb{N}$, and $\tau \in \mathbb{N}$ fixed. Define $a(n)=$ $\sum_{t=n-\tau}^{n-1} \mathds{1}(t \in A)$. Then for all $T \in \mathbb{N}$ and $s \in \mathbb{N}$ we have the inequality:
     \begin{align}
       \sum_{n=1}^T \mathds{1}(n \in A, a(n) \leq s) \leq s\lceil T / \tau\rceil .  
     \end{align}
\end{restatable}
